# Supplementary material for: Strange metal state near a heavy-fermion quantum critical point
Source: arXiv:1701.04599 source file (2017-01-17)
Supplement: Supplementary file 1 [file Supp-YRS-0116-2017.pdf]

# Supplementary Materials for "Strange metal state near a heavy-fermion quantum critical point"

Yung-Yeh, Chang[1], Silke Paschen[2], and Chung-Hou Chung[1,3]

[1] *Department of Electrophysics, National Chiao Tung University, 1001 University Rd., Hsinchu, 300 Taiwan, R.O.C.*

[2] *Institute of Solid State Physics, TU Vienna, Wiedner Hauptstrasse 8-10, 1040 Vienna, Austria*

[3] *Physics Division, National Center for Theoretical Sciences, HsinChu, 300 Taiwan, R.O.C.*

(Dated: January 17, 2017)

## A. LAGRANGE MULTIPLIER $\lambda$, OBSERVABLES AND LOCAL CONSTRAINT FOR $N = 1,\ S = 1/2$ LOCAL IMPURITY

For $N = 1$ ($Sp(1) \cong SU(2)$) and $S = 1/2$, the constraint for the local impurity operator $f_{i\sigma}$ on the $i$-th site becomes $\sum_\sigma f^\dagger_{i\sigma} f_{i\sigma} = 1$, where $i$ is the site index while $\sigma =\uparrow, \downarrow$ denotes spin. Including the constraints, a total Hamiltonian can be in general expressed as

$$\begin{aligned} H' =& H_0 + H_I + \lambda(f^\dagger f - 1) \\ =& H_0 + H_I + \lambda Q, \end{aligned} \tag{A.1}$$

where $Q \equiv f^\dagger f$ is the number operator of the pseudo–fermion $f$ at $i$-th site. Here, $H_0$ denotes the non-interacting Hamiltonian, $H_I$ contains all the interaction terms and $\lambda$ is the Lagrange multiplier which could be also regarded as the chemical potential of $f$. It is known that in this case only one particle is allowed to stay on one lattice site [1–3], which, on the other hand, implies $\lambda$ should be sent to infinity. To justify the condition of infinite $\lambda$ for the case of singly occupation, we first analyze the partition function for arbitrary value of $Q$ and $\lambda$, given by

$$Z_\lambda = \sum_Q \langle \{Q\}| e^{-\beta(H+\lambda Q)} |\{Q\}\rangle = \sum_Q Z(Q) e^{-\beta\lambda Q} \tag{A.2}$$

where $Z(Q) = \langle\{Q\}|e^{-\beta H}|\{Q_i\}\rangle$ with $H \equiv H_0 + H_I$. However, only states with $Q = 1$ is of physical interest here, i.e. $Z(Q = 1)$. Meanwhile, $\lambda$ should be sent to infinity at the end of calculation. The partition function of physical interest reads

$$\begin{aligned} \lim_{\lambda\to\infty} \frac{\partial Z_\lambda}{\partial \xi} &= \lim_{\lambda\to\infty} \sum_Q \left[ Z(Q) Q\, e^{\beta\lambda(-1+Q)} \right] \\ &= \lim_{\lambda\to\infty} e^{\beta\lambda} \langle Q\rangle_\lambda Z(1) \\ &= Z(1), \end{aligned} \tag{A.3}$$

where $\xi = \exp(-\beta\lambda)$. After sending $\lambda$ to infinity, we indeed obtain the partition function only involving $Q = 1$ on each sites as shown in Eq. (A.3) . Via Eq. (A.3), the expectation value of a physical observable $O$ is defined as

$$\langle O\rangle_{phys} = \frac{\mathrm{Tr}\left[Oe^{-\beta H}\right]_{Q=1}}{Z(1)} \tag{A.4}$$

Note that the numerator of $\langle O\rangle_{phys}$ could be alternatively written as

$$\begin{aligned}\mathrm{Tr}\left[Oe^{-\beta H}\right]_{Q=1} = \lim_{\lambda\to\infty}\frac{\partial\langle O\rangle_\lambda}{\partial\xi} &= \lim_{\lambda\to\infty}\sum_Q\langle\{Q\}|OQe^{-\beta H}|\{Q\}\rangle e^{-\beta\lambda(Q-1)}\\ &= \lim_{\lambda\to\infty} e^{\beta\lambda}\sum_Q\langle\{Q\}|OQe^{-\beta(H+\lambda Q)}|\{Q\}\rangle\\ &= \lim_{\lambda\to\infty} e^{\beta\lambda}\langle OQ\rangle_\lambda Z(1)\\ &= \lim_{\lambda\to\infty} e^{\beta\lambda}\langle O\rangle_\lambda Z(1).\end{aligned} \tag{A.5}$$

Plugging Eq.(A.3) and Eq.(A.5) into Eq.(A.4), and cancelling $Z(1)$ and $e^{\beta\lambda}$ lead to the expression of $O$ in the presence of the constraint $\sum_{\sigma=\uparrow,\downarrow} f^\dagger_{i\sigma}f_{i\sigma}=1$, which takes the following form:

$$\langle O\rangle_{phys} = \lim_{\lambda\to\infty}\frac{\langle O\rangle_\lambda}{\langle Q\rangle_\lambda}. \tag{A.6}$$

## B. RESCALING OF THE FERMI WAVEVECTOR $k_F$

In this section, we discuss the issue on the rescaling of Fermi wavevector $k_F$ under RG transformation. Our RG scheme is the same as in Ref. [4]. We shall prove that, for the case of $z=d=2$ with $z$ being the dynamical exponent and $d$ being the dimension, the wavevectors for boson and fermion share the same scaling dimension. Therefore, we do not need to apply the patch RG scheme as being used in Ref. [5].

In the following, we take the action for free bosons with the dynamical exponent $z=2$ as an example:

$$S_b = \int^{\Lambda_q} d^dq\, d\omega\, \phi_b^\dagger\left(-i\omega+q^2\right)\phi_b, \tag{B.1}$$

where the subscript $b$ in Eq. (B.1) denotes *boson* here, $\phi_b$ represents the boson field and $\Lambda_q$ denotes the momentum cut-off for bosons. $\mathbf{q}$ and $\omega$ are denoted as the boson wavevector and frequency, respectively. The momentum and frequency are rescaled according to $\omega' = e^{[\omega]l}\omega$ and $\mathbf{q}' = e^{[\mathbf{q}]l}$, where $[\omega]$ and $[\mathbf{q}]$ is defined as the scaling dimension for $\omega$ and $\mathbf{q}$, respectively. Demanding the that $S_b$ should be form invariant after mode elimination, we obtain $2[q]=[\omega]=z=2$. On the other hand, the free fermion action is expressed as

$$S_f = \int^{\Lambda_k} d^dk\, d\epsilon\, \Psi_f^\dagger\left[i\epsilon - \frac{k_F}{m}(|\mathbf{k}|-k_F)\right]\Psi_f, \tag{B.2}$$

where the subscript $f$ in Eq. (B.2) has been used to denote *fermion*. Here, we denote $\mathbf{k}$ as the wavevector (to distinguish fermion wavevector $k$ from $q$ for boson), $m$ the mass, $\epsilon$ the frequency, $\Psi_f$ the fermion field, $k_F$ the Fermi wavevector, $v_F \equiv k_F/m$ the Fermi velocity and $\Lambda_k$ the momentum cut-off for fermions. The frequency $\epsilon$ and momentum $k$ are rescaled via: $\epsilon' = e^{[\epsilon]l}\epsilon, \quad \mathbf{k} = e^{[\mathbf{k}]l}\mathbf{k}$. Furthermore, we also impose the rescaling of Fermi wavevector such that $[\mathbf{k}] = [k_F]$. The condition of scale invariance for $S_f$ implies that the two terms in the square bracket of $S_f$ must be also scale invariant, yielding

$$
\begin{aligned}
& ie^{-[\epsilon]l}\epsilon' - e^{-[\mathbf{k}]l}e^{[m]l}\left(\frac{k'_F}{m'}\right) \times e^{-[\mathbf{k}]l}\left(|\mathbf{k}'| - k'_F|\right) \\
=& e^{-[\epsilon]l}\left[i\epsilon' - e^{-2[\mathbf{k}]l+[\epsilon]l+[m]l}\left(\frac{k'_F}{m'}\right)\left(|\mathbf{k}'| - k'_F\right)\right]
\end{aligned}
\tag{B.3}
$$

Thus, we have $[m] = 2[\mathbf{k}] - [\epsilon]$. Setting $[m] = 0$ leads to $2[k] = [\epsilon]$. For a mixed fermion-boson system, it is reasonable to take $[\omega] = [\epsilon]$, giving rise to $[\mathbf{k}] = 1$. As a result, we have $[\mathbf{k}] = [\mathbf{q}]$, i.e. fermion and boson wavevector have the same scaling dimension.

There exists a fundamental difference between the scaling scheme being in Ref. [5] and ours. Fermi wavevector $k_F$ in Ref. [5] is considered to be scale invariant by Luttinger theorem, the conservation of Fermi volume under RG. This leads to difficulty to maintain the scale invariance for the case of mixed boson fermion systems. To better illustrate this issue, we could a 2–fermion–1–boson interaction with the following action

$$
S_{b-f} = g\int d\omega d\epsilon \int^{\Lambda_k} d^dk \int^{\Lambda_q} d^dq \left[\Psi_f^\dagger(\mathbf{k}+\mathbf{q};\omega+\epsilon)\Psi_f(\mathbf{k};\omega)\phi_b(\mathbf{q};\epsilon)\right]\Theta(\Lambda_k - |\mathbf{k}+\mathbf{q}| + k_F),
\tag{B.4}
$$

where $g$ denotes the coupling constant for the interaction term in Eq. (B.4). After mode elimination via $\Lambda_k \to \Lambda_k e^{-[k]l}$ and $\Lambda_q \to \Lambda_q e^{-[q]l}$, $S_{b-f}$ becomes

$$
\begin{aligned}
S_{b-f} = g\int d\omega d\epsilon \int^{\Lambda_k e^{-l[k]}} d^dk \int^{\Lambda_q e^{-l[q]}} d^dq \left[\Psi_f^\dagger(\mathbf{k}+\mathbf{q};\omega+\epsilon)\Psi_f(\mathbf{k};\omega)\phi_b(\mathbf{q};\epsilon)\right] \\
\times \Theta(\Lambda_k e^{-l[k]} - |\mathbf{k}+\mathbf{q}| + k_F).
\end{aligned}
\tag{B.5}
$$

After rescaling $S_{b-f}$ in Eq. (B.5) back to its original form via the scaling transformation $k' = e^{[k]l}k, \quad q' = e^{[q]l}q$, it is clear that the situation where $k_F$ is not rescaled leads to some difficulities for the case of $z \geq 2$: the difficulty comes from fact that the $\Theta$ function in Eq.

B.5 is not scale invariant. Consequently, we have to seek for another method– the patch RG as shown in Ref. [5] to overcome the difficulty. However, if we allow $k_F$ to be rescaled as we discussed before, the boson and fermion wavevector would have the same scaling dimension. Hence, we do not need to follow the patch RG formalism within our RG scheme.

## C. BARE SCALING DIMENSIONS

In this section, we provide detailed derivations on the bare scaling dimensions of various operators and coupling constants based on the scale invariance of Eq. (1) in the maintext. Note that in what follows we use $k(\omega)$ to simultaneously denote the wavevector (frequency) for both fermions and bosons since it is shown that their wavevectors (frequencies) share the same scaling dimension.

At first, $k$ and $\omega$ are rescaled in the following way:

$$k' = e^l k; \quad \omega' = e^{zl}\omega, \tag{C.1}$$

where $z = 2$ is the dynamical exponent.

The scale invariance of the free field action $S_0$ involving the conduction electron operator $c_k$ in Eq. (1) of the maintext implies

$$c'_{k'} = e^{-(z+d/2)l} c_k. \tag{C.2}$$

Likewise, the bare scaling dimension of the pseudo–fermion operator $f_{k\sigma}$ is determined from the free-field action $S_0$ involving $f_{k\sigma}$. $\lambda$ in $S_0$ is the Lagrange multiplier, we set $\lambda$ to be a scaling invariant quantity, i.e. $[\lambda] = 0$ (In fact, $\lambda \to \infty$ for $N = 1\,(Sp(1)$ and $S = 1/2)$). This result is also consistent with the fact that in the strong $J_\Phi$ but small $J_\chi$ regime, $f-$electron is localized, which preserves the constraint for the local $f-$electrons. Via $[\lambda] = 0$, we have

$$[f_{k\sigma}] = -\frac{d+z}{2}. \tag{C.3}$$

Due to the quadratically dispersed band structures for the Kondo fluctuation field $\hat{\hat{\chi}}$ and the spin-singlet RVB fluctuation $\hat{\hat{\Phi}}$, the scaling dimension of $\hat{\hat{\chi}}$ and $\hat{\hat{\Phi}}$ are found to be the same with that for the conduction electron, namely

$$[c_k] = [\hat{\hat{\chi}}_k] = [\hat{\hat{\Phi}}_k] = -(z + \frac{d}{2}). \tag{C.4}$$

Referring to the action $S_K$ in Eq. (1) of the maintext, $[J_\chi]$ is computed through

$$[J_\chi] + 2d + 2z - \left(z + \frac{d}{2}\right) - \left(z + \frac{d}{2}\right) - \frac{d+z}{2} = 0 \quad \Rightarrow [J_\chi] = \frac{z-d}{2}. \tag{C.5}$$

The scaling dimension of $J_\Phi$ can be determined from the action $S_J$ in Eq. (1):

$$2d + 2z + [J_\Phi] + 2[f] + [\hat{\hat{\Phi}}_k] = 0 \quad \Rightarrow \; [J_\Phi] = -\frac{d}{2}. \tag{C.6}$$

Similarly, for the coupling constant $u_\chi$ for the quartic term of $\hat{\hat{\chi}}_k$, we have

$$[u_\chi] + 3 \cdot (d+z) - 4 \cdot (z + \frac{d}{2}) = 0 \quad \Rightarrow \; [u_\chi] = z - d. \tag{C.7}$$

Since the quartic term for the $\hat{\hat{\Phi}}_k$-field shares the same form for that of $\hat{\hat{\chi}}_k$, therefore, $[u_\Phi] = [u_\chi] = z - d$.

The bare scaling dimension for the single particle density of state per spin can be determined via

$$\int d^d k \propto \int k^{d-1}\, dk \propto \int m^{\frac{d-1}{2}} \epsilon_c^{\frac{d-1}{2}} \left(\frac{dk}{d\epsilon_c}\right) d\epsilon_c, \tag{C.8}$$

where $\epsilon_c = \frac{k^2}{2m}$ denotes the dispersion of itinerant electrons and $m^*$ denotes the mass of itinerant electrons. At the Fermi level,

$$\Rightarrow \int m^{\frac{d-1}{2}} \left(\frac{k_F^2}{m^*}\right)^{\frac{d-1}{2}} \left(\frac{m}{k_F}\right) d\epsilon_c = \int N_0\, d\epsilon_c, \tag{C.9}$$

where $N_0 \equiv N_0(k_F) \propto m\, k_F^{d-2}$ is the single particle, single spin density of states [4]. Thus, under rescaling, the $N_0(k_F)$ transforms as

$$N_0(l, k_F') = e^{(d-z)l}\, N_0(l = 0, k_F). \tag{C.10}$$

It is clear that $N_0(k_F)$ is scaling invariant for $z = d = 2$ within our RG scheme.

## D. GREEN'S FUNCTION FOR THE LOCAL $f$-ELECTRON

In this section, we compute the Green's functions for the local $f$-electrons and the value of the Lagrange multiplier $\lambda$ via the $Sp(N)$ mean-field approach in the FL* phase. In the FL* state, the mean-field Hamiltonian for the local $f$-electrons on a square lattice is given by

$$H_f = \sum_{\mathbf{k}\alpha} \lambda\, f^\dagger_{\mathbf{k}\alpha} f_{\mathbf{k}\alpha} + \sum_{\mathbf{k},\alpha\beta} \left[Q(\mathbf{k})\epsilon_{\alpha\beta} f^\alpha_{\mathbf{k}} f^\beta_{-\mathbf{k}} + h.c.\right] \equiv \sum_{\mathbf{k}} \Psi^\dagger_{\mathbf{k}} \mathcal{M}_{\mathbf{k}} \Psi_{\mathbf{k}}, \tag{D.1}$$

where $Q(\mathbf{k}) = Q_0 \sum_i e^{i\mathbf{k}\cdot\delta_i} = 2Q_0 (\cos k_x a + \cos k_y a) = Q(\text{-}\mathbf{k})$ on a square lattice with $Q_0$ being a constant prefactor and $a$ being defined as the lattice constant here, $\Psi_{\mathbf{k}} = \left( f_{\mathbf{k}\uparrow} \, , \, f^{\dagger}_{-\mathbf{k}\downarrow} \right)$ is a two-component Nambu spinor and

$$\mathcal{M}_{\mathbf{k}} = \begin{bmatrix} -\lambda & -(Q(\mathbf{k})^* + Q(\text{-}\mathbf{k})^*) \\ -(Q(\mathbf{k}) + Q(\text{-}\mathbf{k})) & \lambda \end{bmatrix}. \tag{D.2}$$

The quasiparticle dispersions $E_{\pm}(\mathbf{k})$ of $\Psi_{\mathbf{k}}$ are the eigenvalues of $\mathcal{M}_{\mathbf{k}}$, given by

$$E_{\pm}(\mathbf{k}) = \pm \sqrt{\lambda^2 + |Q(\mathbf{k}) + Q(-\mathbf{k})|^2} \approx \pm\sqrt{\lambda^2 + 64|Q_0|^2} \equiv \pm\bar{\lambda}. \tag{D.3}$$

In the second line of Eq. (D.3), we take the continuous limit $|\mathbf{k}|a \ll 1$. Thus, $Q(\mathbf{k}) \approx 4Q_0 - Q_0(|\mathbf{k}|a)^2 \approx Q_0$. Here, we keep the leading order term $Q_0$ in $Q(\mathbf{k})$. The higher order terms from the expansion of $Q(\mathbf{k})$ in the limit $|\mathbf{k}a| \ll 1$ generates more irrelevant terms due to higher powers of $\mathbf{k}$.

To estimate the value of $\lambda$, we minimize the free energy $F$ of the $f$-electrons w.r.t. the Lagrangian multiplier $\lambda$ (or the chemical potential) and obtain the occupation number $N_f(\lambda)$ of the $f$-electron per site, given by

$$N_f(\lambda) = -\frac{1}{N_s}\frac{\partial F}{\partial \lambda} = \frac{1}{N_s}\left( \sum_{\mathbf{k}} \frac{\lambda}{\sqrt{\lambda^2 + 16Q_0^2(\cos k_x a + \cos k_y a)^2}} \right), \tag{D.4}$$

where $N_s$ denotes the numbers of sites and the $F = -H_f$ is the free energy for the local f-electrons at zero temperature. In the large-$N$ formulation of a quantum antiferromagnet, the constraint $\langle \sum_\alpha f^{\dagger}_{i\alpha} f_{i\alpha} \rangle = 2NS$ should be imposed on each lattice sites. For $N = 1 (Sp(1) \cong SU(2))$ and $S = 1/2$, we plot $N_f(\lambda)$ v.s. $\lambda$ with $S = 1/2$ (or $\kappa \equiv 2S = 1$), shown in Fig. 1. The value of $\lambda$ is obtained via the intersection of $N_f(\lambda)$ curve and the constraint $f(\lambda) = 2S$ (see Fig. 1). It is clear that $\lambda \to \infty$ for the case of $S = 1/2$ (or $\kappa = 1$). We expect a large but finite value of $\lambda$ for the case of the quantum disordered FL* phase where $S < 1/2$ (or $\kappa < 1$), as illustrated in Fig. 1.

The bare normal Green function $G^b_f$ and the anomalous Green function $\mathcal{F}^b_f$ are defined respectively as :

$$G^b_f(\mathbf{k}, \tau) = -\left\langle T_\tau f_{\mathbf{k}\uparrow}(\tau) f^{\dagger}_{\mathbf{k}\uparrow}(0) \right\rangle, \quad \mathcal{F}^b_f(\mathbf{k}, \tau) = -\left\langle T_\tau f^{\dagger}_{-\mathbf{k}\downarrow}(\tau) f^{\dagger}_{\mathbf{k}\uparrow}(0) \right\rangle, \tag{D.5}$$

where the subscript $b$ in Eq. (D.5) denotes *bare*. In frequency space, they are written as

$$G^b_f(\mathbf{k}, \omega_n) = \frac{i\omega_n + \lambda}{(i\omega_n)^2 - \bar{\lambda}^2}, \quad \mathcal{F}^b_f(\mathbf{k}, \omega_n) = -\frac{4Q_0}{(i\omega_n)^2 - \bar{\lambda}^2}. \tag{D.6}$$

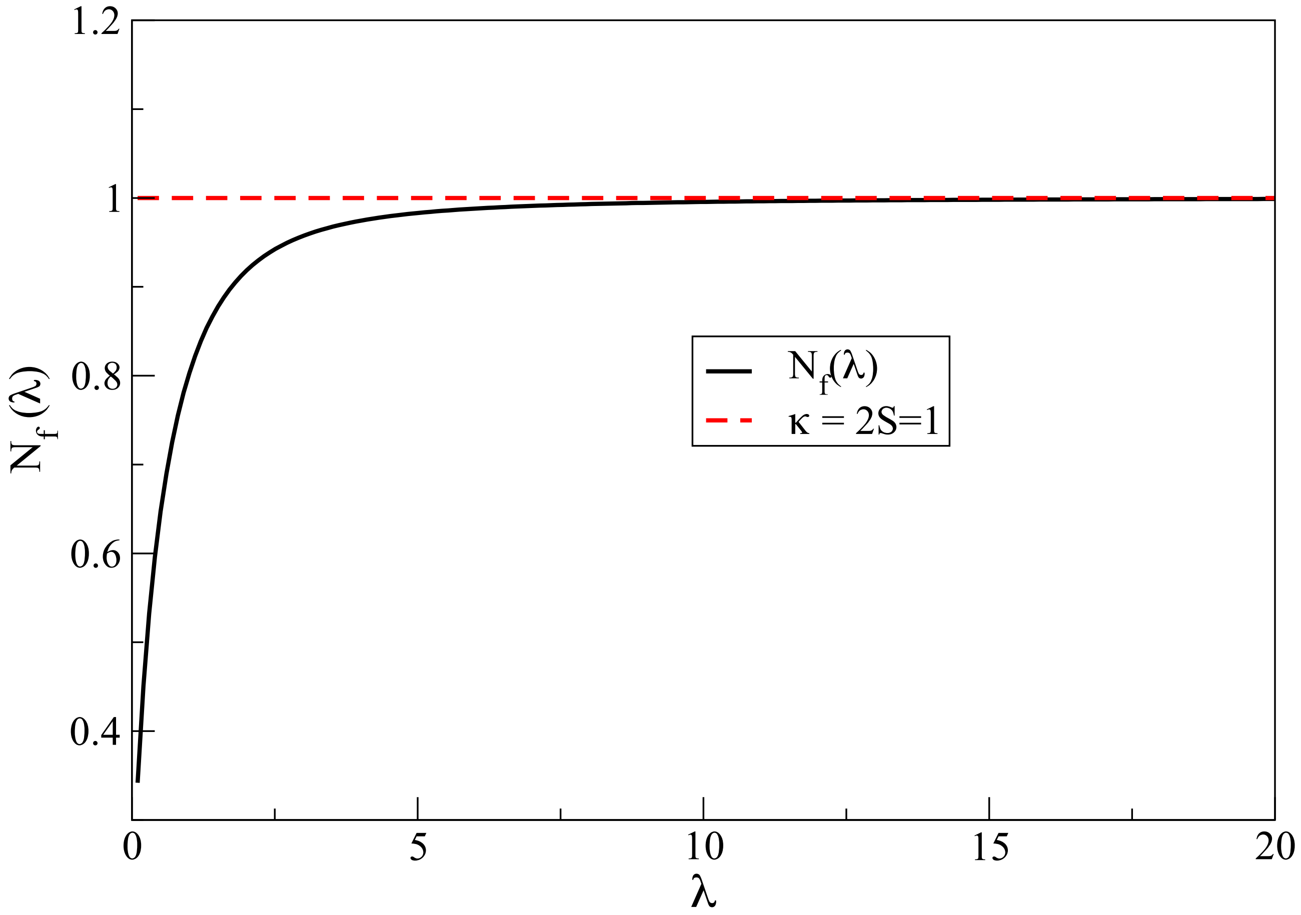


FIG. 1: The black solid curve in the plot shows the occupation number $N_f(\lambda)$ of the $f$-fermions per site with $Q_0 = 0.35$, while the red dashed-line depicts the value of $2S$ under the constraint $\sum_\alpha \langle f^\dagger_{i\alpha} f_{i\alpha}\rangle = 2S$ with $S = 1/2$ on each sites. The intersect of the black curve and the dashed-line in the plot indicates the value of $\lambda$ for the case of $\kappa \equiv 2S = 1$ for $N = 1$ ($Sp(1)$).

In the local limit $\lambda \gg Q_0$, the normal Green function can be further simplified :

$$G^b_f(\mathbf{k}, \omega_n) = \frac{i\omega_n + \lambda}{(i\omega_n)^2 - (\bar{\lambda})^2} \approx \frac{1}{i\omega_n - \bar{\lambda}}, \tag{D.7}$$

while the anomalous Green function vanishes. It is obvious that $G^b_f$ is $\mathbf{k}$ independent and can be regarded as the Green's function for a particle in a flat band.

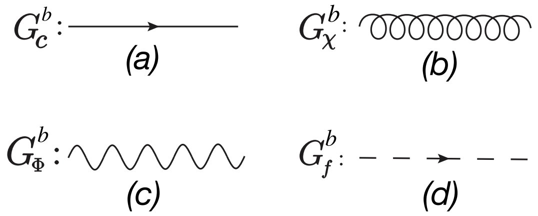


FIG. 2: This plot shows the bare propagators of (a) the conduction electrons $c_k$ (the solid line), (b) the fluctuating Kondo correlation $\hat{\hat{\chi}}_k$ fields (the helical line), (c) the fluctuating RVB spin-singlet $\hat{\hat{\Phi}}_k$ fields (the wavy line) and (d) the local $f$-electrons (the dashed line).

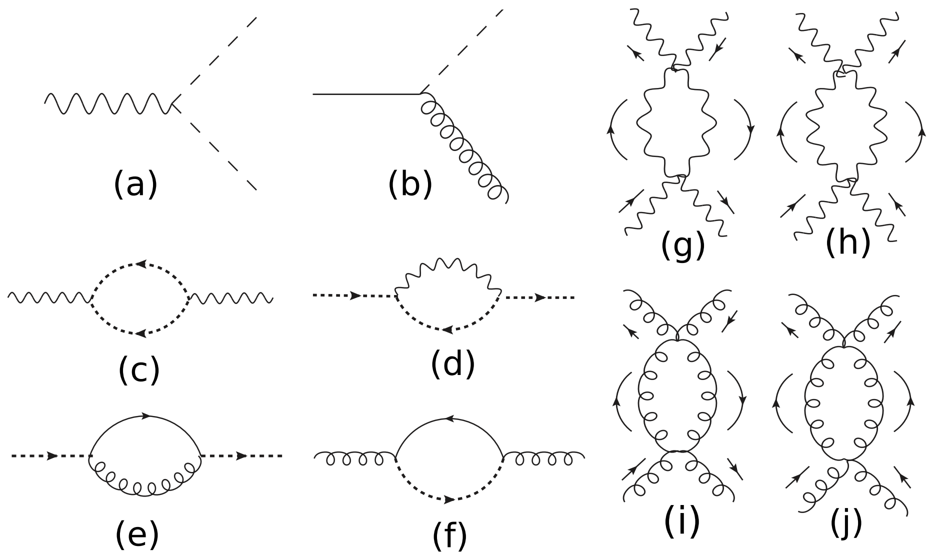


FIG. 3: The interaction vertices for (a) the anti-ferromagnetic RKKY coupling $J_\Phi$, and (b) for the Kondo coupling $J_\chi$. The self–energy diagrams to the one-loop order of (c) the $\hat{\hat{\Phi}}$ field, (d)–(e) the $f$–electron and (f) the $\hat{\hat{\chi}}$ field. The diagrams of the vertex correction to the one-loop order for the quartic terms are shown in (g)–(i) : (g) and (h) for the $u_\Phi$ coupling while (i) and (j) for the $u_\chi$ coupling. Here, the solid, dashed, wavy and helical lines stand for propagators of conduction electrons, local $f$ electrons, the $\hat{\hat{\Phi}}$-field and the $\hat{\hat{\chi}}$-field, respectively.

## E. RG ANALYSIS

### E.1. Self–energy correction

In this section, we derive the one-loop RG $\beta$-functions for various couplings for our model.

Fig. 2 shows diagrammatic representations for various bare propagators:

$$G_c^b(\omega,\mathbf{k}) = \frac{1}{i\omega - \epsilon_c(\mathbf{k})} \quad ; \quad G_f^b(\omega,\mathbf{k}) = \frac{1}{i\omega - \bar{\lambda}}$$
$$G_{\chi,\Phi}^b(\omega,\mathbf{k}) = \frac{1}{i\omega - \epsilon_{\chi,\Phi}(\mathbf{k}) - m_{\chi,\Phi}} + \frac{1}{i\omega + \epsilon_c(\mathbf{k}) - m_{\chi,\Phi}}. \tag{E.1}$$

First, we calculate the one-loop correction to the self-energy of the spin-singlet fluctuation field $\hat{\tilde{\Phi}}_k$. The first contribution comes from Fig. 3–(c), given by

$$\Sigma_\Phi^{(1)}(\tau) = -\frac{8}{2!} \cdot J_\Phi^2 G_f^b(\tau) G_f^b(\tau), \tag{E.2}$$

where $0 < \tau < \beta$. The bare Green's function of the $f$–electron, $G_f^b$, in terms of imaginary time $\tau$ is defined as

$$G_f^b(\tau) = e^{-\bar{\lambda}\tau}\left[(n_F(\bar{\lambda}) - 1)\Theta(\tau) + n_F(\bar{\lambda})\Theta(-\tau)\right] = e^{-\bar{\lambda}\tau}\left[n_F(\bar{\lambda}) - 1\right], \tag{E.3}$$

where $\Theta(\tau)$ is the unit–step function and $n_F(y) = \left(e^{\beta y} + 1\right)^{-1}$ is the Fermi-Dirac distribution function. After taking $\bar{\lambda} \to \infty$, $\Sigma_\Phi(\tau)$ vanishes, i.e. $\Sigma_\Phi^{(1)}(\tau) = 0$.

The self-energy corrections $\Sigma_f$ to the one-loop order for the $f$-electrons are contributed from the two Feynman diagrams as illustrated in Fig. 3-(d) and -(e). The first contribution $\Sigma_f^{(1)}$ as shown in Fig. 3-(d) is given by

$$\begin{aligned}
\Sigma_f^{(1)}(i\omega) =& -\frac{8 \cdot J_\Phi^2}{2! \cdot \beta} \sum_{i\nu} \sum_{\mathbf{k}} G_\Phi^b(-i\omega - i\nu,\ \mathbf{k}) G_f^b(i\nu) \\
=& \frac{4J_\Phi^2}{\beta} \sum_{i\nu,\mathbf{k}} \left[\frac{1}{i\omega + i\nu + \epsilon_\Phi(\mathbf{k}) + m_\Phi} - \frac{1}{i\omega + i\nu - \epsilon_\Phi(\mathbf{k}) - m_\Phi}\right] \cdot \frac{1}{i\nu - \bar{\lambda}} \\
=& -4J_\Phi^2 \sum_{\mathbf{k}} \left[\frac{n_B(\epsilon_\Phi(\mathbf{k}) + m_\Phi) + 1}{i\omega + \epsilon_\Phi(\mathbf{k}) + m_\Phi + \bar{\lambda}} - \frac{n_B(\epsilon_k + m_\Phi)}{i\omega - \epsilon_\Phi(\mathbf{k}) - m_\Phi + \bar{\lambda}}\right],
\end{aligned} \tag{E.4}$$

where, $\omega$ being the fermionic Matsubara frequency and $n_B(y) = (e^{\beta y} - 1)^{-1}$ being the Bose–Einstein distribution. Setting $i\omega = \omega - \bar{\lambda}$ and taking the limit $\bar{\lambda} \to \infty$ at the end, we have, in the low temperature limit

$$\Sigma_f^{(1)}(\omega - \bar{\lambda}) = -4J_\Phi^2 \int_{m_\Phi}^{m_\Phi + \Lambda} d\epsilon \, \frac{1}{\omega + \epsilon} \approx -4J_\Phi^2 \ln\frac{\Lambda}{\omega}. \tag{E.5}$$

Note that $\Sigma_f^{(1)}$ also contributes to the RG $\beta$-function for $1/\Gamma$ via the following approach: $\Sigma_f^{(1)} \propto \ln(\Lambda/\omega) \approx \omega \ln\Lambda - \omega \ln\Lambda + \ln\Lambda \approx \omega \ln\Lambda + \ln\Lambda$ ($\omega \ll \Lambda$). It is clear from Eq. (E.5) that the self-energy of the diagram Fig. 3-(d) contributes a logarithmic divergence.

In addition, the contribution from Fig. 3–(e) is given by

$$\Sigma_f^{(2)}(i\omega) = -\frac{2J_\chi^2}{\beta}\sum_{i\nu}\sum_{k} G_c^b(i\nu,\mathbf{k})G_\chi^b(i\omega - i\nu,\mathbf{k})$$
$$= -\frac{2J_\chi^2}{\beta}\sum_{i\nu,\mathbf{k}}\frac{1}{i\nu-\epsilon_c(\mathbf{k})}\left[\frac{1}{i\omega - i\nu - \epsilon_\chi(\mathbf{k}) - m_\chi} - \frac{1}{i\omega - i\nu + \epsilon_\chi(\mathbf{k}) + m_\chi}\right]. \quad \text{(E.6)}$$

Here, the approximate $\epsilon_c(\mathbf{k}) \pm \epsilon_\chi(\mathbf{k}) \approx \epsilon_c(\mathbf{k})$ is used since $\epsilon_\chi(\mathbf{k})$ compared with $\epsilon_c(\mathbf{k})$ is a higher order term, i.e. $\epsilon_\chi(\mathbf{k}) \ll \epsilon_c(\mathbf{k})$. Thus,

$$\Sigma_f^{(2)}(i\omega) = 2J_\chi^2\sum_{\mathbf{k}}\frac{1}{i\omega - \epsilon_c(\mathbf{k})} = 2J_\chi^2 N_0\int_{-\Lambda}^{\Lambda}\frac{d\epsilon}{i\omega-\epsilon} \sim (\ln\Lambda)^0\,. \quad \text{(E.7)}$$

Therefore, Fig. 3-(e) gives no logarithmic divergence. Finally, Fig. 3-(f) which contributes to the self-energy of $\hat{\bar{\chi}}$, is given by

$$\Sigma_\chi(i\omega) = \frac{2J_\chi^2}{2!\cdot\beta}\sum_{i\nu}\sum_{\mathbf{k}} G_f^b(i\omega + i\nu)G_c^b(i\nu - \epsilon_k) = J_\chi^2\sum_{k}\frac{1}{i\omega + \epsilon_c(\mathbf{k}) - \bar{\lambda}}. \quad \text{(E.8)}$$

Following the similar approach, we have

$$\Sigma_\chi(\omega + \bar{\lambda}) = J_\chi^2 N_0\int_{-\Lambda}^{\Lambda} d\epsilon\,\frac{n_F(\epsilon)}{\omega+\epsilon} \approx -J_\chi^2 N_0 \ln\frac{\Lambda}{\omega}, \quad \text{(E.9)}$$

which leads to a logarithmic divergence.

### E.2. Corrections from the quartic terms

We can further add the quartic terms for the boson fields beyond Gaussian fluctuation into our model. The action for the quartic terms reads

$$\mathcal{S}_4 = \frac{u_\chi}{2}\int dk_1dk_2dk_3\hat{\bar{\chi}}^\dagger_{k_1}\hat{\bar{\chi}}^\dagger_{k_2}\hat{\bar{\chi}}_{k_3}\hat{\bar{\chi}}_{k_1+k_2-k_3} + \frac{u_\Phi}{2}\int dk_1dk_2dk_3\hat{\bar{\Phi}}^\dagger_{k_1}\hat{\bar{\Phi}}^\dagger_{k_2}\hat{\bar{\Phi}}_{k_3}\hat{\bar{\Phi}}_{k_1+k_2-k_3}, \quad \text{(E.10)}$$

where $u_\Phi$ and $u_\chi$ are the coupling constants. The Feynman diagrams of the one-loop vertex correction to $u_\Phi$ and $u_\chi$ are shown in Fig. (3). The vertex correction from the contribution of Fig. 3-(i) gives

$$\Gamma_\chi^{(i)}(i\omega) = -\frac{1}{2}\cdot\frac{1}{4}\cdot 16\cdot\frac{u_\chi^2}{\beta}\sum_{\mathbf{k},i\nu}\left[\frac{1}{i\nu - \epsilon_\chi(\mathbf{k}) - m_\chi} - \frac{1}{i\nu + \epsilon_\chi(\mathbf{k}) + m_\chi}\right]$$
$$\times\left[\frac{1}{i\nu + i\omega - \epsilon_\chi(\mathbf{k}) - m_\chi} - \frac{1}{i\nu + i\omega + \epsilon_\chi(\mathbf{k}) + m_\chi}\right]. \quad \text{(E.11)}$$

Since $0 < \epsilon_\chi(\mathbf{k}) < \Lambda$, $n_B(\epsilon_\chi(\mathbf{k})) \approx 0$ at the low temperature limit. Via the relation $n_B(-y) = -[1+n_B(y)]$, we therefore have

$$\Gamma_\chi^{(i)}(\omega) = -2u_\chi^2 \sum_{\mathbf{k}} \frac{4\epsilon_{\mathbf{k}}}{(i\omega)^2 - 4\epsilon_{\mathbf{k}}^2} = 2u_\chi^2 \ln\frac{\Lambda}{\omega} + \cdots, \tag{E.12}$$

where $[\cdots]$ in the above equation represents the terms which do not contribute logarithmic divergences. Similarly, the logarithmic contribution from Fig. 3-(j) is given by

$$\Gamma_\chi^{(j)}(\omega) = u_\chi^2 \ln\frac{\Lambda}{\omega}. \tag{E.13}$$

Since the Lagrangian of the quartic term for $\hat{\hat{\Phi}}$-boson takes the same form with $\hat{\hat{\chi}}$, therefore, we expect the vertex corrections from Fig. 3-(g) and -(h) share the same results with the contributions from Fig. 3-(i) and -(j), respectively. Namely,

$$\Gamma_\Phi^{(g)}(\omega) = 2u_\Phi^2 \ln\frac{\Lambda}{\omega}; \quad \Gamma_\Phi^{(h)}(\omega) = u_\Phi^2 \ln\frac{\Lambda}{\omega}. \tag{E.14}$$

### E.3. The RG $\beta$-functions

The RG $\beta$-functions are readily obtained via the diagrammatic perturbation approaches, which include renormalizations of the bare interaction vertices (or the coupling constants) and the fields (or the Green's functions) [1, 2]:

$$G_\alpha(\Lambda') = Z_\alpha G_\alpha(\Lambda), \qquad \gamma_J(\Lambda') = Z_J^{-1}\gamma_J(\Lambda),$$

where $G_{\alpha=f,\Phi,\chi}$ and $Z_{\alpha=f,\Phi,\chi}$ denote the Green's function and the field-renormalization factor of the local $f-$fermions, $\hat{\hat{\Phi}}$- and $\hat{\hat{\chi}}$-fields, respectively. Here, the vertex function $\Gamma_J(\omega)$ for the coupling $J$ is in general expressed as $\Gamma_J(\omega) \equiv J\gamma_J(\omega)$ with the corresponding renormalization factor $Z_J$. Here, $J$ represents various couplings such as $J_\Phi$, $J_\chi$ or $u_\chi$. The renormalization of coupling constants are given by

$$\begin{aligned} j_\chi &= Z_{J_\chi} Z_f^{-\frac{1}{2}} Z_\chi^{-\frac{1}{2}} J_\chi, \;\; j_\Phi = Z_{J_\Phi} Z_f^{-1} Z_\Phi^{-\frac{1}{2}} J_\Phi \\ u_\chi &= Z_{u_\chi} Z_\chi^{-2} u_\Phi^0, \qquad u_\Phi = Z_{u_\Phi} Z_\Phi^{-2} u_\Phi^0. \end{aligned} \tag{E.15}$$

The coupling constants $j_{\Phi,\chi}$, $u_{\Phi,\chi}$ ($J_{\Phi,\chi}$, $u^0_{\Phi,\chi}$) in Eq. (E.15) represents the renormalized (bare) couplings. The various $Z-$factors for the renormalized fields and couplings are found

to be (see Section E E.1 and E E.2)

$$Z_f = 1 + 4j_\Phi^2 \cdot d\ln\Lambda, \quad Z_\chi = 1 + j_\chi^2 \cdot d\ln\Lambda,$$
$$Z_{J_\chi} = Z_{J_\Phi} = Z_\Phi = 1, \tag{E.16}$$

where $\Lambda$ is the energy cutoff within the momentum-shell RG. By Eqs. (E.15) and (E.16), the RG $\beta$-functions can be obtained:

$$\frac{d\,j_\Phi}{dl} = -\frac{d}{2}j_\Phi + 4j_\Phi^3\ , \ \frac{d\,j_\chi}{dl} = -\left(\frac{d-z}{2}\right)j_\chi + \frac{1}{2}j_\chi^3 + 2j_\Phi^2 j_\chi,$$
$$\frac{du_\chi}{dl} = -(d-z)u_\chi - 4j_\chi^2 u_\chi - 3u_\chi^2, \quad \frac{du_\Phi}{dl} = -(d-z)u_\Phi - 3u_\Phi^2,$$
$$\frac{d}{dl}\left(\frac{1}{\Gamma}\right) = -z\left(\frac{1}{\Gamma}\right) + 4j_\Phi^2, \quad \frac{dm_\chi}{dl} = zm_\chi + j_\chi^2\ , \ \frac{dm_\Phi}{dl} = zm_\Phi, \tag{E.17}$$

where $d\ln\Lambda = -dl$ is used. To derive the RG $\beta$-function for $m_\chi$ in Eq. (E.17), we define $\tilde{m}_\chi \equiv m_\chi^0 + \Sigma_\chi$ where $\Sigma_\chi$ is given in Eq. (E.9) and $\tilde{m}_\chi$ is a scale-dependent mass. Via the momentum shell RG procedures, we lower the energy cutoff via $\Lambda \to e^{-dl}\Lambda$ with $0 < dl \ll 1$ (it is equivalent to integrating over the high energy modes, i.e. $e^{-dl}\Lambda < \epsilon < \Lambda$). Thus, $\tilde{m}_\chi$ becomes

$$\tilde{m}_\chi = m_\chi^0 + J_\chi^2 dl. \tag{E.18}$$

In the above equation, $d\ln\Lambda = -dl$ is used. Imposing the condition that the mass $\tilde{m}_\chi$ should follow the same scaling behavior of the bare mass $m_\chi$ after integrating out the high energy modes yields

$$m_\chi(dl) = e^{zdl}\tilde{m}_\chi = (1+zdl)(m_\chi^0 + j_\chi^2 dl)$$
$$\Rightarrow \frac{dm_\chi}{dl} = zm_\chi + j_\chi^2. \tag{E.19}$$

Following the similar approach, we can find $m_\Phi$ and $1/\Gamma$. Since the one-loop order correction to $\hat{\hat{\Phi}}$ vanishes, there is no higher order terms in the RG $\beta$-function for $m_\Phi$. To obtain $\beta(1/\Gamma)$, we should use the self-energy of the local $f$-electrons, $\Sigma_f^{(1)} = -4J_\Phi^2 \ln\Lambda$.

To make contact with experiments, we expect the coupling $g \equiv g_0 - J_\Phi/J_\chi$ to play the role of magnetic field $B$ in experiments near the FL$^*$-LFL quantum phase transition. We shall justify our expectation later in Section E E.4. Here the constant $g_0$ can be determined via the condition of $g = 0$ at zero field. The RG $\beta$-function for $g$ is given by

$$\beta\left(g_0 - \frac{J_\Phi}{J_\chi}\right)\Bigg|_{J_\chi = J_\chi^*} = \frac{d}{2}(g_0 - g) - 4J_\chi^{*2}(g_0 - g)^3. \tag{E.20}$$

In Eq. (E.20), we assume the dominant effect of tuning the magnetic field is the change of $J_\Phi$ while $J_\chi$ is closed to its critical value $J_\chi^*$ before reaching the ground state. Thus, we fixed $J_\chi$ at $J_\chi^*$ while deriving the RG $\beta$-function $\beta(g)$. Via the condition $\beta(g_c) = 0$, the fixed point for Eq. (E.20) is given by $g_c = g_0 - \sqrt{d/8J_\chi^{*2}}$. Linearizing $\beta(g)$ near $g_c$ yields

$$\partial\beta(g)/\partial g|_{g=g_c} = d. \tag{E.21}$$

Consequently, the correlation length exponent in this approach is found to be the same as obtained by the inverse of the leading relevant eigenvalues of the linearized RG $\beta$-functions in Eq. (2).

### E.4. RG $\beta$-functions near the quantum critical point $\mathbf{C}_r$

The above RG analysis as in Eq. E.17 is controlled only near the weak coupling fixed point $j_\Phi = 0 = j_\chi$. In order to more precisely locate the QCP at finite values of $j_\Phi$ and $j_\chi$, we obtain the RG scaling equations near the intermediate coupling fixed points $P$ and $Q$. To be more specific, near the fixed point $P$, $j_\chi$ is fixed at $j_\chi = j_\chi^* = \sqrt{\eta}$. Fixing $j_\chi$ at $j_\chi^*$ effectively leads to a shift in the bare scaling dimension of the pseudo $f$-electron, i.e. $[f] \to [f] - \frac{\eta}{4}$, and the bare scaling dimension of the Kondo fluctuating $\hat{\tilde{\chi}}$ boson: $[\hat{\tilde{\chi}}] \to [\hat{\tilde{\chi}}] - \frac{\eta}{4}$. The change in the scaling dimension of the $f$-electron also leads to a change in the scaling dimension of $\bar{\lambda}$ and $J_\Phi$: $[J_\Phi] \to [\tilde{J}_\Phi] = [J_\Phi] + \frac{\eta}{2}$ (See the $S_J$ term in Eq. (1) of the maintext) and $[\bar{\lambda}] \to [\bar{\lambda}] + \frac{\eta}{2}$ (See the $S_0$ term in Eq. (1) of the maintext). Hence, the RG $\beta$-function for $j_\Phi$ near $P$ is replaced by $\tilde{j}_\Phi$ :

$$\frac{d\tilde{j}_\Phi}{dl} = \left(-\frac{d}{2} + \frac{\eta}{2}\right)\tilde{j}_\Phi + 4\tilde{j}_\Phi^3. \tag{E.22}$$

The fixed point value for $\tilde{j}_\Phi$ has now became $\tilde{j}_\Phi^* = \sqrt{z/8}$. Here, the higher order corrections in $\eta$ for the RG $\beta$-functions due to the changes in the bare scaling dimension of $f$ and $\hat{\tilde{\chi}}$ are neglected in Eq. (E.22).

Likewise, near the fixed point $Q$, $j_\Phi$ is fixed at $j_\Phi^* = \sqrt{d/8}$, resulting in a change in the scaling dimension of the $f$-electron: $[f] \to [f] + d/4$ and $[j_\chi] \to [j_\chi^*] = [j_\chi] - \frac{d}{4}$. The corresponding RG $\beta$-function of the Kondo coupling $\tilde{j}_\chi$ (relative to fixed $j_\Phi$) is given by:

$$\frac{d\tilde{j}_\chi}{dl} = -\left(\frac{\eta}{2} + d/4 - 2(j_\Phi^*)^2\right)\tilde{j}_\chi + \frac{1}{2}\tilde{j}_\chi^3. \tag{E.23}$$

The fixed point of Eq. (E.23) is found to be $\tilde{j}_\chi^* = \sqrt{\eta}$. Based on above analysis, the critical point $C_r$ in Fig. 2 in the maintext, which controls the FL*-LFL QPT, is located at the intersect of the two RG $\beta$-functions in Eq. (E.22) and Eq. (E.23): $(\tilde{j}_\chi^{2*}, \tilde{j}_\Phi^{2*}) = (\eta, z/8)$.

To closely investigate the behaviors of the RG flow near $C_r$, we linearize the RG $\beta$-functions for $\tilde{j}_\Phi$ and $\tilde{j}_\chi$ in Eq. (E.22) and Eq. (E.23). Expressing $\tilde{j}_{\chi,\,\Phi} = \tilde{j}^*_{\chi,\,\Phi} + \delta\tilde{j}_{\chi,\,\Phi}$ and taking the leading order contributions of $\delta\tilde{j}_{\chi,\,\Phi}$, the linearized RG $\beta$-functions $\beta(\delta\tilde{j}_{\chi,\,\Phi})$ for $\tilde{j}_{\chi,\,\Phi}$ near $C_r$ are given by

$$\begin{aligned}\begin{pmatrix}\beta(\delta\tilde{j}_\chi)\\ \beta(\delta\tilde{j}_\Phi)\end{pmatrix} &= \begin{pmatrix}\frac{\partial\beta(\tilde{j}_\chi)}{\partial\tilde{j}_\chi} & \frac{\partial\beta(\tilde{j}_\chi)}{\partial\tilde{j}_\Phi}\\ \frac{\partial\beta(\tilde{j}_\Phi)}{\partial\tilde{j}_\chi} & \frac{\partial\beta(\tilde{j}_\Phi)}{\partial j_\Phi}\end{pmatrix}\Bigg|_{\tilde{j}_{\chi,\,\Phi}=\tilde{j}^*_{\chi,\,\Phi}} \begin{pmatrix}\delta\tilde{j}_\chi\\ \delta\tilde{j}_\Phi\end{pmatrix}\\ &= \begin{pmatrix}-\frac{\eta}{2}-\frac{d}{4}+2\,j_\Phi^{*2}+\frac{3}{2}\,\tilde{j}_\chi^{*2} & 0\\ 0 & -\frac{d}{2}+\frac{\eta}{4}+12\,\tilde{j}_\Phi^{*2}\end{pmatrix}\begin{pmatrix}\delta\tilde{j}_\chi\\ \delta\tilde{j}_\Phi\end{pmatrix}\\ &= \begin{pmatrix}\eta & 0\\ 0 & z\end{pmatrix}\begin{pmatrix}\delta\tilde{j}_\chi\\ \delta\tilde{j}_\Phi\end{pmatrix}\end{aligned} \tag{E.24}$$

For convenience, we may define

$$\mathcal{M} \equiv \begin{pmatrix}\eta & 0\\ 0 & z\end{pmatrix} \tag{E.25}$$

From the linearized RG $\beta$-functions near $C_r$, we see that the critical exponent for the correlation length $\nu = 1/z$ which is obtained from the inverse of the leading eigenvalues of the matrix $\mathcal{M}$ in Eq. (E.25).

## F. DISPERSION FOR THE COMPOSITE BOSON FIELDS

The dispersions for the composites boson fields, $\hat{\chi}$ and $\hat{\hat{\Phi}}$, are obtained via integrating out the $c$-electron away from the Fermi surface. This approach is equivalent to including the self energy correction to the Green functions of the $\hat{\chi}$ and $\hat{\hat{\Phi}}$ bosons in the Dyson equation $G^{-1} = G^{b^{-1}} - \Sigma$ via random phase approximation (RPA). The dispersion of $\hat{\chi}$ is the real part of its self-energy $\Sigma_\chi$ (see Fig. 3-(f)):

$$\begin{aligned}\mathrm{Re}\Sigma_\chi(\mathbf{k},\,\omega\to 0) &= \mathrm{Re}\left(N_0 J_\chi^2\left(\int_{\Lambda-\epsilon_c(\mathbf{k})}^{\Lambda} + \int_{-\Lambda}^{-\Lambda+\epsilon_c(\mathbf{k})}\right)\frac{n_f(\epsilon')\,d\epsilon'}{\omega+\epsilon'-\bar{\lambda}+i\delta}\right)\Bigg|_{\omega\to 0}\\ &\approx N_0 J_\chi^2 \ln\left[1+\frac{-\frac{k^2}{2m^*}+\Lambda}{\bar{\lambda}}\right] \approx N_0 J_\chi^2\left[-\left(\frac{k^2}{2m^*\bar{\lambda}}\right)+\frac{\Lambda}{\bar{\lambda}}\right].\end{aligned} \tag{F.1}$$

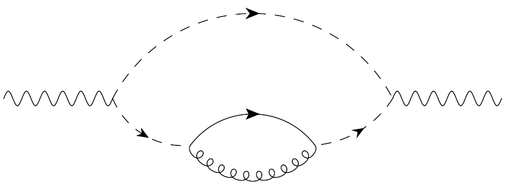

FIG. 4: The self energy diagram in RPA contributed to the dispersion of $\hat{\hat{\Phi}}_k$-field. Various propagators shown in this figure are defined in Fig. 2.

Here, $\epsilon_c(\mathbf{k}) = k^2/2m^*$ and the Taylor expansion of $\ln(1+x) \approx x$ for $x = \frac{-\frac{k^2}{2m^*}+\Lambda-\omega}{\bar{\lambda}} \ll 1$. Note that after integrating out the high energy modes of the $c$-electron, the self-energy of $\hat{\hat{\chi}}$ will simultaneously renormalize its frequency $\omega$, mass and dispersion. However, the term proportional to $\omega/\bar{\lambda}$ which corresponds to the renormalized frequency, can be neglected since $\omega/\bar{\lambda} \ll 1$. Also, $N_0 J_\chi^2 \Lambda/\bar{\lambda}$ can be absorbed into the mass $m_\chi$ of the $\hat{\hat{\chi}}$ field and leads to a redefinition of $m_\chi$.

Meanwhile, the imaginary part of $\Sigma_\chi$ is

$$\begin{aligned}\mathrm{Im}\Sigma_\chi =&\mathrm{Im}\left(N_0 J_\chi^2 \left(\int_{\Lambda-\epsilon_c(\mathbf{k})}^{\Lambda} + \int_{-\Lambda}^{-\Lambda+\epsilon_c(\mathbf{k})}\right) \frac{n_f(\epsilon^{'})\, d\epsilon^{'}}{\omega+\epsilon^{'}-\bar{\lambda}+i\delta}\right)\\ =&-\pi N_0 J_\chi^2 \int_{-\Lambda}^{-\Lambda+\epsilon_c(\mathbf{k})} \delta(\omega+\epsilon^{'}-\bar{\lambda}) d\epsilon^{'} = 0.\end{aligned} \tag{F.2}$$

The above integration vanishes since $\bar{\lambda}-\omega \gg 0$. Note that $\mathrm{Im}\Sigma_\chi = 0$ we found here implies $\hat{\hat{\chi}}$ bosons do not show Landau damping. As a result, the Fermi surface volume exhibits a "jump" instead of a smooth crossover across the QCP, consistent with the experiment in Ref. [6, 7].

Similarly, the dispersion for $\hat{\hat{\Phi}}$-boson comes from $\mathrm{Re}\Sigma_\Phi$. However, since the $\Sigma_\Phi$ at second order of $J_\Phi$ vanishes in Sec. E E.1, the first non-trivial contribution comes from the fourth order in $J_\Phi^2\, J_\chi^2$ as shown in the RPA diagram of Fig. 4, which is given by

$$\mathrm{Re}\Sigma_\Phi(\omega\to 0) = -\left.\frac{2J_\Phi^2}{\bar{\lambda}+\mathrm{Re}\Sigma_f^{(2)}(\omega)}\right|_{\omega\to 0}, \tag{F.3}$$

where

$$\mathrm{Re}\Sigma_f^{(2)}(\mathbf{k},\,\omega\to 0) = 2N_0 J_\chi^2 \left(\int_{-\Lambda}^{-\Lambda+\epsilon_c(\mathbf{k})} + \int_{\Lambda-\epsilon_c(\mathbf{k})}^{\Lambda}\right) \left.\frac{d\epsilon}{\omega-\epsilon}\right|_{\omega\to 0} \approx \frac{N_0 J_\chi^2}{m^*\Lambda}\, k^2. \tag{F.4}$$

Thus, we have

$$\begin{aligned}\mathrm{Re}\Sigma_f^{(2)}(\mathbf{k},\,\omega\to 0) =& -\frac{2J_\Phi^2}{\bar\lambda}\left(\frac{1}{1+\frac{N_0\,J_\chi^2}{m^*\,\bar\lambda(\Lambda+\omega)}\,k^2}\right)\Bigg|_{\omega\to 0}\\ \approx& -\frac{2J_\Phi^2}{\bar\lambda}+\frac{2N_0J_\chi^2J_\Phi^2}{m^*\,\bar\lambda^2\,\Lambda}\,k^2+\mathcal{O}(\frac{\omega}{\bar\lambda^2}).\end{aligned} \tag{F.5}$$

According to the Dyson equation, the dispersion for $\hat{\hat{\Phi}}$ is given by $\frac{2N_0J_\chi^2J_\Phi^2}{m^*\,\bar\lambda^2\,\Lambda^2}\,k^2$. The renormalized mass for the $\hat{\hat{\Phi}}_{\mathbf{k}}$ boson to the fourth order is given by

$$\begin{aligned}m_\Phi &= J_\Phi-\Sigma_\Phi(\omega=0)=J_\Phi+\frac{2J_\Phi^2}{\bar\lambda+\Sigma_f^{\prime(2)}(\omega\to 0)}\\ &=J_\Phi+\frac{1}{2}\frac{J_\Phi^2}{\bar\lambda+4J_\chi^2aN_0\ln\Lambda}=-\frac{2}{\bar\lambda^3}J_\Phi^2J_\chi^4\,\ln\Lambda+\cdots\,,\end{aligned} \tag{F.6}$$

where $a=\epsilon_\chi(\mathbf{k})/\epsilon_c(\mathbf{k})=N_0J_\chi^2/\bar\lambda$. In the last line of the above equation, $[\cdots]$ denotes the terms which do not give logarithmic divergences. In the above, $N_0$ can be absorbed into $\bar\lambda$. To extract the non-zero logarithmic divergence of $m_\Phi$, we should evaluate $\Sigma_f^{\prime(2)}$ which is the next leading contribution of $\Sigma_f^{(2)}$ as shown in Eq. (E.7) and (E.7). Starting from the third line in Eq. (E.6), we have

$$\begin{aligned}\Sigma_f^{\prime(2)}(i\omega) &= -2J_\chi^2\sum_{\mathbf{k}}\left[\frac{n_F(\epsilon_c(\mathbf{k}))}{i\omega-\epsilon_c(\mathbf{k})-\epsilon_\chi(\mathbf{k})}-\frac{n_F(\epsilon_c(\mathbf{k}))}{i\omega-\epsilon_c(\mathbf{k})+\epsilon_\chi(\mathbf{k})}\right]\\ &+2J_\chi^2\sum_{\mathbf{k}}\left[\frac{n_F(i\omega-\epsilon_\chi(\mathbf{k}))}{i\omega-\epsilon_c(\mathbf{k})-\epsilon_\chi(\mathbf{k})}-\frac{n_F(i\omega+\epsilon_\chi(\mathbf{k}))}{i\omega-\epsilon_c(\mathbf{k})+\epsilon_\chi(\mathbf{k})}\right]\\ &=-4J_\chi^2a\sum_{\mathbf{k}}\frac{\epsilon_c(\mathbf{k})n_F(\epsilon_c(\mathbf{k}))}{(i\omega-\epsilon_c(\mathbf{k}))^2}.\end{aligned} \tag{F.7}$$

Taking $i\omega\to\omega+i\delta$ with $\delta\to 0$ leads to

$$\begin{aligned}\Sigma_f^{\prime(2)}(\omega) &= -4J_\chi^2aN_0\int_{-\Lambda}^{0}\frac{\epsilon_c d\epsilon_c}{(\omega-\epsilon_c+i\delta)^2}\approx -4J_\chi^2aN_0\int_{-\Lambda}^{0}\frac{\epsilon_c d\epsilon_c}{(\omega-\epsilon_c)^2}\\ &=4J_\chi^2aN_0\int_{\omega+\Lambda}^{\omega}\frac{\omega-v}{v^2}\,dv=4J_\chi^2aN_0\ln\frac{\Lambda}{\omega}+\cdots\,.\end{aligned} \tag{F.8}$$

In above equation, the change of variable $v\equiv\omega-\epsilon_c$ is used.

## G. $T_{LFL}$ AND $T_{FL^*}$ AND $T^*$

In this section, we evaluate three crossover temperature scales $T_{FL^*}$, $T_{LFL}$ and $T^*$. Moreover, we will show the difficulty to experimentally observe the FL* phase by taking the ratio $T_{FL^*}/T_{LFL}$ near the QCP.

To estimate $T_{FL^*}$ in the FL$^*$ phase near the QCP where $J_\chi$ is fixed at its fixed point value at $P$ and the mean-field value of the Kondo correlation $\chi_i$ is absent, we integrate out the $\hat{\tilde{\chi}}_{\mathbf{k}}$-boson and the conduction electron $c_{\mathbf{k}}$ for the fluctuation part of the Lagrangian, which generates a self energy for the pseudo f-electron as shown in Section E E.1:

$$\begin{aligned}\Sigma_f^{(2)}(\omega) =& -2J_\chi^2 N_0 \int_{-\Lambda}^{\Lambda} \frac{d\epsilon_c}{\omega - \epsilon_c - m_\chi + i\delta} \\ =& -2J_\chi^2 N_0 \left[\mathcal{P}\int_{-\Lambda}^{\Lambda} \frac{d\epsilon_c}{\omega - \epsilon_c - m_\chi} - i\pi \int_{-\Lambda}^{\Lambda} d\epsilon_c \delta(\omega - \epsilon_c - m_\chi)\right] \\ =& ik_0, \end{aligned} \tag{G.1}$$

where $k_0 =\equiv 2\pi N_0 J_\chi^2$ denotes the imaginary part in $\Sigma_f^{(1)}$. Taking this imaginary part $k_0$ into account, $\Sigma_f^{(1)}$ becomes

$$\Sigma_f^{(1)}(\omega) = -4J_\Phi^2 \int_0^{\Lambda} \frac{d\epsilon}{\omega + \epsilon - ik_0}, \tag{G.2}$$

Thus, $ik_0$ term in Eq. (G.2) effectively generates a cutoff (an unit step function) in the RG $\beta$- function for $J_\Phi$ [8, 9]:

$$\frac{d\Sigma_f^{(1)}(\omega - \bar{\lambda})}{d\ln\Lambda} = -4J_\Phi^2 \Theta(\Lambda - k_0) \tag{G.3}$$

From the above equation, the RG $\beta$-function for $j_\Phi$ acquires a lower cutoff $k_0 = 2\pi N_0 J_\chi^2$. To calculate $T_{FL^*}$, we first linearize the RG $\beta$-function for $j_\Phi$ near the QCP. Let us define $j \equiv \tilde{j}_\Phi - \tilde{j}_\Phi^*$ where $\tilde{j}_\Phi^* = \sqrt{z/8}$, the linearized RG $\beta$-function for $\tilde{j}_\Phi$ near the fixed point $P$ becomes

$$\frac{dj}{d\ln\Lambda} = -\left(-\frac{z}{2} + 12\tilde{j}_\Phi^{*2}\right) j = -z\, j \tag{G.4}$$

For convenience, we differentiate $j$ by $\ln\Lambda$ where $\Lambda$ is the running energy cutoff in the momentum shell RG. Solving the above equation by integrating over $\Lambda$ from the lowest energy scale $k_0$ leads to

$$\ln\frac{j}{j_0} = -z\int_{k_0}^{\Lambda} d\ln\Lambda' = \ln\left(\frac{\Lambda}{k_0}\right)^{-z} \Rightarrow \frac{j}{j_0} = \left(\frac{\Lambda}{k_0}\right)^{-z}, \tag{G.5}$$

The correlation length $\xi \sim 1/\Lambda$ is introduced at which $j \sim \mathcal{O}(1)$ via Eq. (G.4) and Eq. (G.5). The correlation length $\xi$ therefore reads

$$\xi = k_0^{-1}\, j_0^{-1/z}. \tag{G.6}$$

The crossover scale $T_{FL^*}$ is estimated via $T_{FL^*} \sim \xi^{-z}$. With the help of the relations $j_0 = \tilde{j}_\Phi - \tilde{j}_\Phi^* \sim (g - g_c)$ and $z = 2$, we finally arrive

$$T_{FL^*} \sim J_\chi \, k_0^2 \, (g - g_c) \propto \; J_\chi^5 \, N_0^2 \, (g - g_c). \tag{G.7}$$

in the FL$^*$ phase near the quantum critical point $C_r$. $T_{FL^*}$ also exhibits linear-in-$g - g_c$ behavior.

To obtain the crossover scale $T_{LFL}$ in the LFL phase where $j_\chi$ is fixed while the $J_K$ term becomes relevant, we have to integrate out the conduction electrons $c_k$ both for the mean-field and the fluctuating parts in the Lagrangian as well as the $\hat{\tilde{\chi}}_\mathbf{k}$ bosons. The contribution from integrating out $c_k$ of the fluctuating part of the Lagrangian gives a lower energy cutoff $k_0 \equiv 2\pi N_0 J_\chi^2$ as shown above. We will show later that this contribution is negligible compared to the other contribution mentioned above. In the case of integrating out the $c_k$ electrons at mean-field level, it would be convenient to adopt the path integral formalism ( see Ref. [10] for details). The partition function for the conduction electrons $c_k$ is given by

$$\int \mathcal{D}[\bar{c}, c] \, e^{-\int d\tau \, \sum_{\mathbf{k}\sigma} \left[ \bar{c}_{\mathbf{k}\sigma}(\partial_\tau + \epsilon_c(\mathbf{k}))c_{\mathbf{k}\sigma} + \chi_\mathbf{k} \bar{f}_{\mathbf{k}\sigma} c_{\mathbf{k}\sigma} + \bar{c}_{k\sigma} f_{\mathbf{k}\sigma} \bar{\chi}_\mathbf{k} \right]}. \tag{G.8}$$

In the path integral formalism, all the quantum fields are regarded as $c$-numbers, so we use say $\bar{c}$ instead of $c^\dagger$ to represent the conjugate field of $c$. The action of $c_{\mathbf{k}\sigma}$ can be schematically expressed as

$$\bar{c} \cdot A \cdot c + \bar{c} \cdot \zeta + \bar{\zeta} \cdot c. \tag{G.9}$$

where the matrix $A \equiv \partial_\tau + \epsilon_c(\mathbf{k})$ which is diagonal in the $c_{k\sigma}$ basis and $\zeta \equiv \chi \bar{f}$. Integrating out the $c$-electron yields

$$Z \propto e^{\bar{\zeta} \cdot A^{-1} \cdot \zeta / 4} \, (\det A)^{-1}, \tag{G.10}$$

where $\bar{\zeta} \cdot A^{-1} \cdot \zeta = \int d\tau \sum_{\mathbf{k}\sigma} \bar{f}_{\mathbf{k}\sigma} \frac{|\chi|^2}{\partial_\tau + \epsilon_c(\mathbf{k})} f_{\mathbf{k}\sigma}$. Integrating out the mean-field conduction electrons leads to a self energy $ik_0'$ with $k_0' = -\pi N_0 |\chi|^2 \, \mathrm{sgn}(\omega)$ for the pseudo f-electrons. Following the same reasoning as shown in Eq. (G.1) and Eq. (G.7), we obtain another lower energy cutoff $\pi N_0 |\chi|^2 \, \mathrm{sgn}(\omega)$ for the RG $\beta$-function of $\tilde{j}_\Phi$. The resulting lower energy cutoff denoted as $\tilde{k}_0$ is the sum of the two, i.e. $\tilde{k}_0 = k_0 + k_0'$. However, in the LFL phase the condensate $\chi$ is relevant relative to fixed $j_\chi = j_\chi^*$ near the QCP C$_r$. As a result, $\tilde{k}_0$ is

dominated by the $\chi$ term. To be more specific, fixing $j_\chi$ at $j_\chi^*$ leads to the shift in the bare scaling dimension of the pseudo $f$-electron, i.e. $[f] \to [f] - \eta/4$, and this also leads to the change in the scaling dimension of the mean-field $\chi$, namely $[\chi] = \eta/4$. Following the same approach as shown above, we have

$$T_{LFL} \sim N_0^2 \, J_\chi \, (J_\chi^*)^{-1} \, |\chi|^4 \, (g - g_c). \tag{G.11}$$

We may estimate the ratio between these two crossover scales: $T_{FL^*}/T_{LFL} \propto J_\chi^4/|\chi|^4$ . As the running cutoff scale $l \to L$ under RG with $L \gg 1$ being the system size, $|\chi/J_\chi| \to L^{\eta/4} \gg 1$ for finite $\eta > 0$. Hence, we expect a negligible ratio: $T_{FL^*}/T_{LFL} \propto L^{-\eta} \ll 1$. This may explain the difficulty in observing $T_{FL^*}$ in experiments [11, 12].

Finally, we estimate the crossover scale $T^*$ between small and large Fermi surface. $T^*$ is identified as the onset of the mean-field $\chi$ field. We may linearize the RG $\beta$-function for $\tilde{j}_\Phi$ in Eq. (E.22) relative to the fixed mean-field variable $\chi$. Note that we treat $J_K$ is marginal and $J_\chi$ is an irrelevant operator here. In the similar way, we integrate out the $c$-electrons in the mean-field Lagrangian and obtain the lower cutoff $\pi N_0 |\chi|^2 \,\mathrm{sgn}(\omega)$ for the RG beta function of $j \equiv \tilde{j}_\Phi - \tilde{j}_\Phi^*$.

$$\frac{d\,j}{d \ln \Lambda} = -\left(-\frac{d}{2} + 12 J_\Phi^{*2}\right) j = -d\,j. \tag{G.12}$$

Following the same route, the small to large Fermi surface crossover $T^*$ is found to be

$$T^* \sim N_0^2 \, \chi \, |\chi|^4 \, (\chi^*)^{-z/d} \, (g - g_c)^{z/d} \approx N_0^2 |\chi|^5 \, (\chi^*)^{-z/d} \, (g - g_c)^{1-\eta/z}. \tag{G.13}$$

where $\chi^*$ denotes the fixed point of $\chi$. Hence, $T^*$ exhibits a sub-linear crossover scale in $g - g_c$. From Eq. (G.11) and (G.13), the ratio $T_{LFL}/T^* \sim J_\chi \, \chi^{-1} \, (g - g_c)^{\eta/z} < 1$ at given $g = g_c^+$, which is consistent with the experiment [11, 12]. This result comes from the fact $\chi$ is relevant relative to fixed $j_\chi$.

## H. PHYSICAL OBSERVABLES

In this section, we provide the details on calculating various physical observables.

### H.1. Specific heat coefficient $\gamma(T)$

We focus on contributions to the electronic specific heat coefficient $C_V(T)/T$ from the two Gaussian fluctuating boson fields $\hat{\tilde{\chi}}$ and $\hat{\tilde{\Phi}}$. Here, we follow the RG procedures for the

free energy $F$ in Ref. [13–15] by considering the renormalization of temperature.

We start with the action for the Gaussian model $S_G$ given by

$$S_G = \beta \sum_{\omega_n} \sum_{\mathbf{k}} \left( \delta + k^2 + \frac{|\omega_n|}{\gamma(\mathbf{k})} \right) \phi_n(\mathbf{k}) \phi_{-n}(-\mathbf{k}), \tag{H.1}$$

where $\phi_n(\mathbf{k})$ represents a general boson field. Since $\phi_n^*(\mathbf{k}) = \phi_{-n}(\text{-}\mathbf{k})$ from the fact that $\phi(\mathbf{r}, \tau)$ is real, we have

$$S_G = \beta \sum_{\omega_n} \sum_{\mathbf{k}} \left( \delta + k^2 + \frac{|\omega_n|}{\gamma(\mathbf{k})} \right) |\phi_n(\mathbf{k})|^2 \tag{H.2}$$

The free energy for the Gaussian model $F_G$ can be computed from the equation $F_G = -\beta^{-1} \ln Z_G$ with $Z_G$ being the partition function, where

$$Z_G = \int \mathcal{D}\phi_n(\mathbf{k})\, e^{-S_G} = \prod_{\omega_n > 0} \prod_{|\mathbf{k}| \geq \Lambda} \frac{\pi}{\beta \left( \delta + k^2 + \frac{|\omega_n|}{\gamma(\mathbf{k})} \right)}. \tag{H.3}$$

Via the above equation for $Z_G$, we have the free energy

$$F_G = -\frac{1}{\beta} \sum_{\omega_n} \sum_{\mathbf{k}} \ln \left( \frac{\pi}{\beta(\delta + k^2 + \frac{|\omega_n|}{\gamma(\mathbf{k}))}} \right) = \frac{V}{\beta} \sum_{\omega_n} \int \frac{d^d k}{(2\pi)^d} \ln \left( \delta + k^2 + \frac{|\omega_n|}{\gamma(\mathbf{k}} \right) + const. \tag{H.4}$$

To perform the Matsubara sum, it would be convenient to take the derivative of $F_G$ with respect to $\delta$, that is

$$\frac{\partial F_G}{\partial \delta} = \frac{V}{\beta} \sum_{\omega_n} \int \frac{d^d k}{(2\pi)^d} \frac{1}{\delta + k^2 + \frac{|\omega_n|}{\gamma(\mathbf{k})}} \tag{H.5}$$

and introduce the following integral:

$$I \equiv \frac{1}{2} \oint_C \frac{dz}{2\pi i} \frac{\coth{(z\beta/2)}}{\delta + k^2 - iz/\gamma(\mathbf{k})} = \frac{1}{2} \oint_C \frac{dz}{2\pi i} f(z). \tag{H.6}$$

The poles of the complex function $f(z)$ come from

① From $\coth(z\beta/2) = (e^{\beta z} + 1)/(e^{z\beta} - 1) = \infty$. It is clear that the poles occur at $z = i2n\pi/\beta = i\omega_n$ where $n \in \mathbb{Z}$. The residue of $\coth(\epsilon\beta/2)$ at $z = i\omega_n$ is $2/\beta$.

② $\delta + k^2 - iz/\gamma(\mathbf{k}) = 0$, thus $z = -i\gamma(\mathbf{k})(\delta + k^2)$. However, we do not need to take this pole into account since $C$ is chosen to enclose on the upper-half complex plane.

The contour integral of $f(z)$ along $C$ is therefore given by

$$I = \frac{1}{\beta} \sum_{\omega_n > 0} \frac{1}{\delta + k^2 + \omega_n/\gamma(\mathbf{k})}. \tag{H.7}$$

Alternatively, the contour integral along $C$ of Eq. (H.6) can be separated into four individual integrals along certain regions on $C$:

$$\begin{aligned} I = \frac{1}{2} \Bigg[ \left( \int_{-R}^{-r} + \int_{r}^{R} \right) \frac{d\epsilon}{2\pi i} \frac{\coth(\epsilon\beta/2)}{\delta + k^2 - i\epsilon/\gamma(\mathbf{k})} + \int_{C_1} \frac{dz}{2\pi i} \frac{\coth(z\beta/2)}{\delta + k^2 - iz/\gamma(\mathbf{k})} \\ + \int_{C_2} \frac{dz}{2\pi i} \frac{\coth(z\beta/2)}{\delta + k^2 - iz/\gamma(\mathbf{k})} \Bigg]. \end{aligned} \tag{H.8}$$

The integral over the contour $C_1$ vanishes since the integrand approaches to zero as the radius $R$ of the contour $C_1$ is taken to be infinity. The first and second terms in Eq. (H.8), which correspond to the integrals along the real axis $\epsilon \equiv Re(z)$, can be combined to form the Cauchy principal value and can be further simplified as

$$\begin{aligned} \frac{1}{2} \mathcal{P} \int_{-\infty}^{\infty} \frac{d\epsilon}{2\pi i} \frac{\coth(\epsilon\beta/2)}{\delta + k^2 - i\epsilon/\gamma(\mathbf{k})} &= \frac{1}{2} \int_{0+}^{\infty} \frac{d\epsilon}{\pi} \frac{\coth(\epsilon\beta/2)\, \epsilon/\gamma(\mathbf{k})}{(\delta + k^2)^2 + (\epsilon/\gamma(\mathbf{k}))^2} \\ &= -\frac{1}{2} \int_{0+}^{\infty} \frac{d\epsilon}{\pi} \coth(\frac{\epsilon\beta}{2})\, \partial_\delta \tan^{-1} \left( \frac{\epsilon/\gamma(\mathbf{k})}{\delta + k^2} \right). \end{aligned} \tag{H.9}$$

In the last line of the above equation, we have applied $\partial_\delta \tan^{-1}\left(\frac{\epsilon/\gamma(\mathbf{k})}{\delta + k^2}\right) = -\frac{\epsilon/\gamma(\mathbf{k})}{(\delta+k^2)^2 + (\epsilon/\gamma(\mathbf{k}))^2}$. Integrating over $\delta$, we reproduce the Gaussian free energy $F_G$ shown in Ref. [14]:

$$F_G = -\frac{V}{2} \int \frac{d^d k}{(2\pi)^2} \int_{0+}^{\gamma(\mathbf{k})} \frac{d\epsilon}{\pi} \coth(\frac{\epsilon\beta}{2}) \tan^{-1} \left( \frac{\epsilon/\gamma(\mathbf{k})}{\delta + k^2} \right). \tag{H.10}$$

The RG $\beta$-functions via Millis' approach in Ref. [14] read

$$\begin{aligned} \frac{dT(l)}{dl} &= zT(l), \\ \frac{d\delta(l)}{dl} &= 2\delta(l) + 2u(l)(n+2) f^{(2)}(T(l),\, \delta(l)), \\ \frac{dF(l)}{dl} &= (d+z)F(l) + f^{(0)}(T(l),\, \delta(l)), \\ \frac{du(l)}{dl} &= [4 - (d+z)]u(l) - 4u^2(l)(n+8) f^{(4)}(T(l), \delta(l)). \end{aligned} \tag{H.11}$$

Here, $n$ is the components of the ordered parameter, $f^{(0)}$, $f^{(2)}$ and $f^{(4)}$ are defined in Ref. [14]. The quantum regime is specified as $\delta(l)$ is renormalized to of order of one, i.e. $\delta(l = l_0) \approx \mathcal{O}(1)$ while the renormalized temperature is small, i.e. $T(l = l_0) = Te^{zl_0} \ll \delta(l_0)$

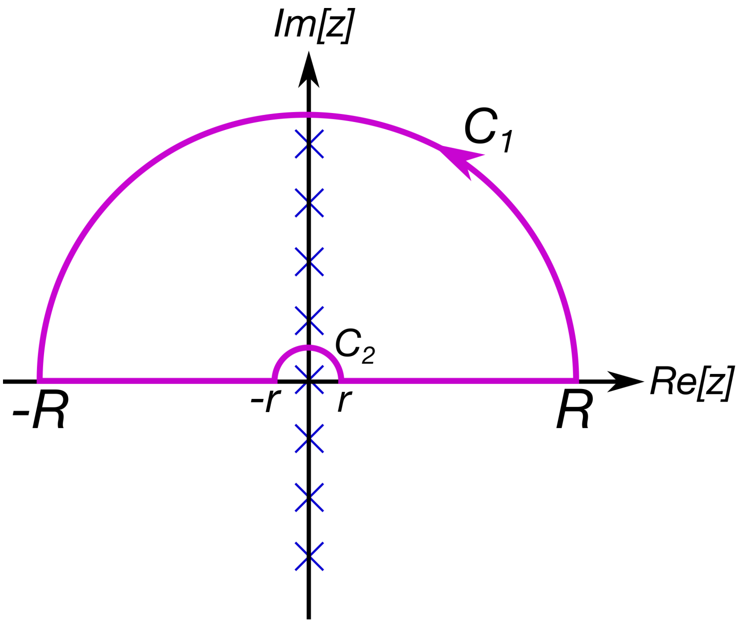


FIG. 5: This figure depicts the contour being chosen to perform the contour integration for the calculation of the Gaussian free energy $F_G$. $R$ and $r$ represent the radius of the larger contour $C_1$ and the smaller one $C_2$, respectively. The symbols "×" denotes the poles.

(the scale $l_0$ is determined via $\delta(l_0) = 1$). At the Gaussian fixed point in the quantum regime, all the renormalized quantities can be obtained by evaluating the expansion of those quantities in powers of $T$ near $T = 0$. Integrating over $l$ to the scale $l_0$ for the RG $\beta$ function of $F(l)$ yields the free energy [14, 15]:

$$F = e^{-(d+z)l_0} F_G(l_0) + F_{SC}, \tag{H.12}$$

where the scale-dependent free energy $F_{SC}$ [14, 15] is defined as

$$F_{SC} = \int_0^{l_0} e^{-(d+z)\,l} f^{(0)}(T\,e^{z\,l})\,dl, \tag{H.13}$$

where $f^{(0)}(T) = F_k^{'} + F_\epsilon^{'}$ with

$$\begin{aligned} F_k^{'} &\equiv V\Lambda^d\Omega_d \int_0^{\gamma(\Lambda)} \frac{d\epsilon}{\pi} \coth\frac{\epsilon}{2T} \tan^{-1}\frac{\epsilon/\gamma(\Lambda)}{(\delta+\Lambda^2)} \\ F_\epsilon^{'} &\equiv \frac{V}{\pi}\int_0^{\Lambda} \frac{d^dk}{(2\pi)^d} \coth\frac{\gamma(\mathbf{k})}{2T} \tan^{-1}\frac{\gamma(\mathbf{k})}{\delta+k^2}. \end{aligned} \tag{H.14}$$

For $d = 2+\eta$, $z = 2$ with $\eta > 0$, only $F_k^{'}$ is important in $f^{(0)}(T)$. Expanding $f^{(0)}(T)$ around

$T=0$, the leading term for $f^{(0)}(T)$ in the quantum regime at is given by

$$\begin{aligned} f^{(0)}(T) &\approx f^{(0)}(T=0) + T\,\frac{df^{(0)}(T)}{dT}\Big|_{T=0} \\ &= f^{(0)}(T=0) + \frac{V\Omega_2}{\pi}\int_0^{1/2T} dx\,\frac{2Tx}{\sinh^2 x}\tan^{-1}(Tx)\Big|_{T=0} \\ &\approx f^{(0)}(T=0) + 2\,\frac{V\Omega_2}{\pi}\left[A_2T^2 - \frac{1}{3}\,A_4T^4\right]. \end{aligned} \tag{H.15}$$

In the above derivation, the L'Hospital's theorem and the expansion $\tan^{-1}x = x - \frac{x^3}{3} + \frac{x^5}{5} + \mathcal{O}(x^7)$ has been used. The coefficients $A_m$ is defined as

$$A_m \equiv \int_0^\infty \frac{x^m}{\sinh^2 x}\,dx. \tag{H.16}$$

The term at $T=0$ gives a negligible contribution to $F_{SC}$. We therefore find

$$\begin{aligned} F_{SC} =& 2\frac{V\Omega_2}{\pi}\int_0^{l_0} dl\left[A_2T^2\,e^{(-d+z)\,l} - \frac{1}{3}A_4T^4\,e^{(-d+3z)\,l}\right] \\ \approx& 2\,\frac{V\Omega_2A_2}{\eta\,\pi}\,T^2\,r^{\frac{\eta}{2}} - \frac{V\Omega_2A_4}{6\pi}\,\frac{T^4}{r^2}, \end{aligned} \tag{H.17}$$

where $r = e^{-l_0/2}$.

On the other hand, the classical regime can be determined through $\delta(l) \approx T(l)/\delta(l) \sim 1$. Following Millis's RG procedures [14], to calculate the renormalized quantities, it is convenient to evaluate the $T > \delta(l_0)$ and $T < \delta(l_0)$ regimes, separately. The result for the classical regime at $d = 2+\eta$ and $z = 2$ is given by

$$F_{SC} = \alpha T^{2+\eta/2} - DTe^{-(2+\eta)\,l_0}. \tag{H.18}$$

Here, the constant value of $\alpha$ is of order of the bandwidth cutoff, i.e. $\alpha \sim \Lambda$ and

$$D = \frac{2\Omega_2}{\pi}\int_0^1 \frac{d\epsilon}{\epsilon}\tan^{-1}\epsilon + \frac{2\Omega_2}{\pi}\int_0^1 k^{1+\eta}\tan^{-1}\frac{1}{k^2}\,dk. \tag{H.19}$$

Note that the term $DTe^{-(2+\eta)l_0}$ in Eq. (H.18) linear in $T$ here does not contribute to the specific heat coefficient $C_V/T$ as $C_V/T \propto \frac{\partial^2 F}{\partial T^2} \to 0$. We will show later that the contribution from the other term $\alpha T^{2+\eta/2}$ in Eq. (H.18) is also negligibly small compared to that from $F_G$.

To proceed, we take an alternative route to compute the Gaussian free energy $F_G$ from the partition function $Z_G$ for the quadratic Gaussian fluctuation Hamiltonian $H_G$, where

$$H_G = \sum_{\mathbf{k}} \hat{\bar{\Phi}}_{\mathbf{k}}(\epsilon_\Phi(\mathbf{k}) + m_\Phi)\hat{\bar{\Phi}}_{\mathbf{k}} + \sum_{\mathbf{k}} \hat{\bar{\chi}}_{\mathbf{k}}(\epsilon_\chi(\mathbf{k}) + m_\chi)\hat{\bar{\chi}}_{\mathbf{k}}, \tag{H.20}$$

which is contributed from the Gaussian fluctuations in $\hat{\hat{\Phi}}$ and $\hat{\hat{\chi}}$. The free energy and the partition function for bosons take the form

$$F_G = -T \ln Z_G, \quad \text{with} \quad Z_G = \mathrm{Tr}\, e^{-\beta H_G}. \tag{H.21}$$

where $\beta = 1/T$. Via Eq. (H.20), the free energy $F_G$ takes the following form

$$\begin{aligned} F_G &= -T \left[ \ln \prod_{\mathbf{k}} \left(1 - e^{-\beta(\epsilon_\Phi(\mathbf{k}) + m_\Phi)}\right)^{-1} + \ln \prod_{\mathbf{k}} \left(1 - e^{-\beta(\epsilon_\chi(\mathbf{k}) + m_\chi)}\right)^{-1} \right] \\ &= T \int_0^{\Lambda_k} \frac{d^d k}{(2\pi)^d} \left( \ln\left(1 - e^{-\beta(\epsilon_\Phi(\mathbf{k}) + m_\Phi)}\right) + \ln\left(1 - e^{-\beta(\epsilon_\chi(\mathbf{k}) + m_\chi)}\right)\right), \end{aligned} \tag{H.22}$$

where $\Lambda_k$ is the upper momentum cutoff. Following Millis' finite temperature RG scenario [14], we may integrate out the fast modes of which the wavevectors laying between $\Lambda_k e^{-l} \leq k \leq \Lambda_k$ with $l > 0$ and maintain the form invariance for Eq. (H.22) by taking the rescalings $k(l) = k e^{l}$ and $T(l) = T e^{zl}$ with $T \equiv T(l=0)$ being the bare temperature. Integrating out the fast modes yields

$$\begin{aligned} F_G &= e^{-(d+z)\,l}\, T(l) \int_0^{\Lambda_k} \frac{d^d k(l)}{(2\pi)^d} \left( \ln\left(1 - e^{-\beta(l)(\epsilon_\Phi(\mathbf{k(l)}) + m_\Phi)}\right) + \ln\left(1 - e^{-\beta(l)(\epsilon_\chi(\mathbf{k(l)}) + m_\chi)}\right)\right) \\ &\quad + F_k' \cdot l \\ &\equiv e^{-(d+z)\,l}\, F_G(l) + + F_k' \cdot l, \end{aligned} \tag{H.23}$$

where $\beta(l) \equiv 1/T(l)$ and the term $F_k' \cdot l$ is the contribution from integrating out the fast modes, which is equivalent to $F_{SC}$ as shown in Eq. (H.13) and thus is neglected as shown later. Apparently, the scaling behaviors of free energy in Eq. (H.23) is identical to Eq. (H.12). To calculate the electronic specific heat, we need the ensemble average of the internal energy $\bar{E}_G$ of the Gaussian fluctuation fields $\hat{\hat{\Phi}}$ and $\hat{\hat{\chi}}$, given by

$$\bar{E}_G = W(J_\Phi) \int_{m_\Phi}^{\Lambda} d\epsilon_\Phi \, \frac{\epsilon_\Phi^{1+\eta/2}}{e^{\beta \epsilon_\Phi} - 1} + W(J_\chi) \int_{m_\chi}^{\Lambda} d\epsilon_\chi \, \frac{\epsilon_\chi^{1+\eta/2}}{e^{\beta \epsilon_\chi} - 1}. \tag{H.24}$$

Here, $V$ denotes the system volume, $\Lambda$ is the upper cutoff energy scale ($\Lambda$ and $\Lambda_k$ are different cutoff scales) while $W(J_\Phi) \equiv V(\Omega_d/2)\left(m^* \bar{\lambda}^2 \Lambda / 4\pi N_0 J_\Phi^2 J_\chi^2\right)^{1+\eta/2}$ and $W(J_\chi) \equiv 2^{\eta/2}\, V \Omega_d \left(m^* \bar{\lambda} / 2\pi N_0 J_\chi^2\right)^{1+\eta/2}$ are constants with $\Omega_d \equiv 2\pi^{d/2}/\Gamma(d/2)$ being the solid angle of a $d$-dimensional sphere ($\Gamma(n)$ denotes the gamma function with argument $n$). Since $W(J_\Phi) \gg W(J_\chi)$ due to the greater power of $\bar{\lambda}$ in $W(J_\Phi)$, the ensemble average of the

internal energy for $\hat{\hat{\chi}}$ is negligible compared to that from $\hat{\hat{\Phi}}$ field. Also, it is clear that $\hat{\hat{\Phi}}$ is much larger that all the prefactors in Eq. (H.17) and Eq. (H.18), we therefore can neglect the $F_{SC}$ term completely. Similar to Eq. (H.23), we may integrate out the higher energy contribution in $\bar{E}_G$, leading to

$$\bar{E}_G = W(J_\Phi) \left( \int_{m_\Phi}^{\Lambda e^{-2l}} + \int_{\Lambda e^{-2l}}^{\Lambda} \right) d\epsilon_\Phi \, \frac{\epsilon_\Phi^{1+\eta/2}}{e^{\beta\epsilon_\Phi} - 1}$$
$$= e^{-(4+\eta)\, l}\, \bar{E}_G(l) + \bar{E}_G' \cdot l, \tag{H.25}$$

where $\bar{E}_G' \cdot l$ can be derived from $F_k' \cdot l$ in Eq. (H.23) and thus the contribution from the term $\bar{E}_G' \cdot l$ will be neglected in the derivation of the specific heat coefficient later. In the above derivation, the scaling for the kinect energy of the $\hat{\hat{\Phi}}$ field follows $\epsilon_\Phi(l) = \epsilon_\Phi \, e^{2l}$ since $\epsilon_\Phi$ is quadratically proportional to $k$, and $m_\Phi(l) = m_\Phi \, e^{2l}$. Finally, the specific heat coefficient $C_V/T$ is obtained by the definition $C_V/T \equiv T^{-1}\partial\bar{E}_G/\partial T$:

$$\frac{C_V}{T} = e^{-\eta l}\, W(J_\Phi) \int_{m_\Phi(l)}^{\Lambda} d\epsilon_\Phi(l) \, \left. \frac{\beta(l)^2\, \epsilon_\Phi(l)^{2+\eta/2}\, e^{\beta(l)\epsilon_\Phi(l)}}{\left(e^{\beta(l)\epsilon_\Phi(l)} - 1\right)^2} \right|_{l=l_0}$$
$$= \frac{1}{4}\, A(l_0) \left(\frac{T}{T_{LFL}}\right)^{\eta/2} \int_{m_\Phi/T}^{m_\Phi\Lambda/T} dx \, \frac{x^{2+\eta/2}}{\sinh^2(x/2)} \tag{H.26}$$

with $x \equiv \epsilon_\Phi(l)/T(l)$ and the scale dependent prefactor $A(l_0) = e^{-\eta l_0} W(J_\Phi)$. The second line in Eq. (H.26) is evaluated near the critical fixed point $C_r$ at which $m_\Phi(l)$ is renormalized to of order of one, $m_\Phi(l_0) \approx \mathcal{O}(1) \Rightarrow 1 = m_\Phi e^{z\, l_0} = m_\Phi \xi^z$ with $m_\Phi$ being the bare mass of the $\hat{\hat{\Phi}}$-field, and $T(l_0) = T e^{z l_0} \sim T\xi^z \sim T/T_{LFL}$. In the above derivations, the relations $e^{l_0} = \xi$ and $\xi^z \sim T_{LFL}^{-1} \sim (g - g_c)^{-1} \sim (J_\Phi - J_\Phi^*)^{-1}$ have been used since near $C_r$ the RG flows along the direction of $J_\Phi$ with $J_\chi$ fixed at $J_\chi^*$ dominates the critical properties (see Section E E.4). The result of the (normalized) specific heat coefficient $\gamma(T/T_{LFL}) \equiv C_V/(A(l_0)T)$ is shown in Fig. 3 in the maintext.

Due the predominant prefactor $W(J_\Phi)$, the corrections to the free energy $F_{SC}$ based on Millis' approach [14, 15] in Eq. (H.17) for the quantum regime and in Eq. (H.18) for the classical regime can be neglected for the calculation of the specific heat coefficient.

### 1. The scaling behavior for $\gamma(T/T_{LFL})$

We now examine the scaling behavior of the prefactor $A(l_0)$ in $\gamma(T/T_{LFL})$. Following the scaling for the free energy in Eq. (H.12), the scaling behavior of the prefactors in front of the normalized specific heat coefficient $\gamma(T/T_{LFL})$ around the fixed point $P$ exhibits

$$A(l_0) \propto e^{-\eta l_0} W(J_\Phi) \propto e^{-\eta\, l_0} \left( \frac{m^* \,\bar{\lambda}^2\, \Lambda}{2N_0 J_\Phi^2 J_\chi^2} \right)^{1+\eta/2}. \tag{H.27}$$

Here, the density of states for $c$-electrons $N_0 \sim m^* k_F^{d-2}$ is invariant under rescaling. Note that we should rescale the Fermi wavevector $k_F$ as $k_F \to k_F/e^{l_0}$, which comes from the rescaling of the free energy $F_G$. However, the energy cutoff $\Lambda$ is invariant under the rescaling. At this stage, the coupling constants such as $J_\Phi$, $J_\chi$ still remain "bare". Moreover, since the specific heat coefficient in the previous section is analyzed around the fixed point $P$ where $J_\chi \to J_\chi\, e^{-\eta l_0/2} \equiv j_\chi(l_0)$, leading to a corresponding change in the bare scaling dimension of $f$ and $\hat{\bar{\chi}}$, i.e. $[f] \to [f] - \frac{\eta}{4}$ and $[\hat{\bar{\chi}}] \to [\hat{\bar{\chi}}] - \frac{\eta}{4}$. Thus, the change in the bare scaling dimension of $f$ makes $\bar{\lambda}$ to acquire an extra scale dimension relative to fixed $j_\chi = j_\chi^*$, namely $\bar{\lambda} \to \bar{\lambda}\, e^{\eta l_0/2}$ (or equivalently $[\bar{\lambda}] \to [\bar{\lambda}] + \eta/2$). In addition, from the RPA calculation of $\epsilon_\Phi(\mathbf{k})$ as shown in Section F, the constant prefactor in $\epsilon_\Phi(\mathbf{k})$ in Eq. (F.5) acquires an extra $e^{2\eta l_0}$ contribution due to the changes in $[f]$ and $[\hat{\bar{\chi}}]$ (This extra contribution $e^{2\eta l_0}$ comes from the bare Greens's functions of $f$ and $\hat{\bar{\chi}}$ in the the RPA diagram as shown in Fig. 4 which contains three Green's functions for $f$ and one for $\hat{\bar{\chi}}$). Collecting all the contributions of $e^{l_0}$ and using the relation $e^{l_0} \sim (g - g_c)^{-1/2}$ yields

$$\begin{aligned} A(l_0) &\propto e^{-\eta\, l_0} W(J_\Phi) \propto (g-g_c)^{\eta/2} \cdot \left( \frac{(g-g_c)^{-\eta/2}}{(g-g_c)^{\eta/2} \cdot (g-g_c)^{\eta}} \right)^{1+\eta/2} \\ &= (g-g_c)^{-\alpha}, \end{aligned} \tag{H.28}$$

where $\alpha = 3\eta/2 + \eta^2$ while experimentally $\alpha \approx 0.33$ [11]. To better match the scaling of the (normalized) specific heat coefficient $\gamma(T/T_{LFL})$ in the power law regime, we choose the optimized value of $\eta \approx 0.18$. In this case, $\alpha$ from our theory is estimated as $\alpha \approx 0.315$, which agrees well with the experiments [11]. The plot for $\gamma(T/T_{LFL})$ is shown in Fig. 3 in the maintext.

*2. Specific heat coefficient $C_V/T$ contributed from the quartic $u_\Phi$ term*

In this subsection, we are going to evaluate the higher order correction for the specific heat coefficient and its scaling behaviors under scaling transformation. At the end, we show that the correction to the specific heat gives a negligible contribution in the scaling regime of our interest.

The higher order correction for the specific heat $\Delta C_V$ contributed from the quartic term $u_\Phi$ can be analyzed as follows [16]:

$$\frac{\Delta C_V}{T} = \frac{\partial\,(\Delta S)}{\partial T}\,, \tag{H.29}$$

where $S$ denotes the entropy. The relation between the entropy and the thermodynamical potential $\Omega$ takes the following form

$$\Delta S = -\frac{\partial\,(\Delta\Omega)}{\partial T},\ \text{where}\ \Omega = -T\ln Z. \tag{H.30}$$

In Eq. (H.30), $Z$ is the grand partition function. Thus, $\Delta\Omega = -T\ln(Z/Z_0)$ with $Z_0$ being the grand partition function in the absence of interaction terms. To analyze the specific heat coefficient $C_V/T$ within the diagrammatic perturbation theory, we need the relation between $Z$ and the $\mathcal{S}$-matrix $\langle\mathcal{S}(\beta)\rangle$, given by

$$Z = Z_0\langle\mathcal{S}(\beta)\rangle, \tag{H.31}$$

where $\langle\mathcal{S}(\beta)\rangle$ is defined as

$$\langle\mathcal{S}(\beta)\rangle = \sum_{n=0}^{\infty}\frac{(-1)^n}{n!}\int_0^\beta d\tau_1\int_0^\beta d\tau_2\cdots\int_0^\beta d\tau_n\langle\mathcal{T}_\tau\hat{H}_{int}(\tau_1)\hat{H}_{int}(\tau_2)\cdots\hat{H}_{int}(\tau_n)\rangle_{closed\ loops}. \tag{H.32}$$

Including the interaction, the thermodynamical potential can be therefore expressed as

$$\Delta\Omega = -T\ \ln\left(\langle\mathcal{S}(\beta)\rangle\right) = -T\ \ln\left(1+\text{diagrams}\right), \tag{H.33}$$

where the $\mathcal{S}$-matrix in Eq. (H.33) is written as a summation over the contributions of all orders of the Feynman diagrams. The leading non-trial diagram, which is of first order in $u_\Phi$, is depicted in Fig. 6, giving rise to the corresponding correction to the $\mathcal{S}$-matrix

$$\begin{aligned}\langle\mathcal{S}(\beta)\rangle^{(1)} &= -\,u_\Phi\int_0^\beta d\tau\sum_{\mathbf{k}_1}G_\Phi(\mathbf{k}_1,\tau=0)G_\Phi(-\mathbf{k}_1,\tau=0)\\ &= -\,\frac{1}{4}\,u_\Phi\,W(J_\Phi)\,\beta^{2-\eta/2}\,F(\beta),\end{aligned} \tag{H.34}$$

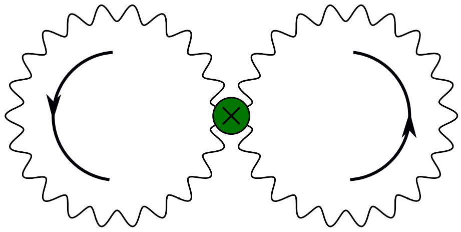

FIG. 6: The Feynman diagram for the lowest leading non-trivial correction from the quartic term $u_\Phi|\hat{\tilde{\Phi}}|^4$ to the specific heat coefficient. The wavy lines represent the the bare propagator of $\hat{\tilde{\Phi}}$ while the filled $\otimes$ symbol denotes the interaction vertex of the quartic term in $\hat{\tilde{\Phi}}$.

where, in the imaginary-time domain, $G_\Phi(\mathbf{k},\tau)$ takes the following form

$$G_\Phi(\mathbf{k},\tau) = -\Theta(\tau)\frac{1}{2\epsilon_\Phi(\mathbf{k})}\left[\left(n_B(\epsilon_\Phi(\mathbf{k}))+1\right)e^{-\tau\epsilon_\Phi(\mathbf{k})} + n_B\left(\epsilon_\Phi(\mathbf{k})\right)e^{\tau\epsilon_\Phi(\mathbf{k})}\right] \tag{H.35}$$

with $\Theta(\tau)$ being the unit step function. The function $F(\beta)$ in Eq. (H.35) is given by

$$F(\beta) \equiv \int_{\beta m_\Phi}^{\beta\Lambda}\frac{dx}{x^{2-\eta/2}}\left[\frac{4}{(e^x-1)^2}+\frac{4}{e^x-1}+1\right]. \tag{H.36}$$

The leading non-trivial correction to $\Delta\Omega^{(1)}$ from the quartic term $u_\Phi$ is therefore given by

$$\begin{aligned}\Delta\Omega^{(1)} &= -\,T\,\langle\mathcal{S}(\beta)\rangle_0^{(1)} = \frac{1}{4}\,u_\Phi\,\beta^{1-\eta/2}\,W(J_\Phi)\,F(\beta)\\ &= e^{z(1-\eta/2)l}\,\Delta\Omega^{(1)}(T(l)),\end{aligned} \tag{H.37}$$

where

$$F(\beta(l)) \equiv \int_{\beta(l)m_\Phi(l)}^{\beta(l)\Lambda}\frac{dx}{x^{2-\eta/2}}\left[\frac{4}{(e^x-1)^2}+\frac{4}{e^x-1}+1\right]. \tag{H.38}$$

The second line in Eq. (H.37) shows the scaling behavior for $\Delta\Omega^{(1)}$ under scale transformation. Following the definition of entropy, the leading correction to the entropy and its corresponding scaling behavior follows

$$\begin{aligned}\Delta S^{(1)}(T) &\equiv -\,\frac{\partial\Delta\Omega^{(1)}}{\partial T} = \frac{u_\Phi\,\beta^{2-\eta/2}\,W(J_\Phi)}{4}\,\left[(1-\frac{\eta}{2})F(\beta)+\beta\,F'(\beta)\right]\\ &= e^{z(2-\eta/2)l}\Delta S^{(1)}(T(l)).\end{aligned} \tag{H.39}$$

where $F'(\beta)\equiv dF(\beta)/d\beta$. Via Eq. (H.39), we obtain the leading non-trivial correction to the specific heat coefficient $\Delta C_V^{(1)}/T \equiv \partial\left(\Delta S^{(1)}\right)/\partial T$, given by

$$\frac{\Delta C_V^{(1)}}{T} = -\frac{1}{4}\,u_\Phi\,\beta^{3-\frac{\eta}{2}}\,W(J_\Phi)\,\left[\left(2-\frac{3\eta}{2}\right)\,F(\beta)+(4-\eta)\beta\,F'(\beta)+\beta^2\,F''(\beta)\right]. \tag{H.40}$$

Likewise, we are able to show $\frac{\Delta C_V^{(1)}}{T}$ exhibits the following scaling behavior:

$$
\begin{aligned}
&\frac{\Delta C_V^{(1)}}{T} = e^{z(2-\eta/2)l} \cdot \frac{\partial T(l)}{\partial T} \cdot \frac{\partial\left(\Delta S^{(1)}(T(l))\right)}{\partial T(l)} \\
&= -\frac{1}{4} u_\Phi \, e^{z(3-\eta/2)l} \, \beta(l)^{3-\eta/2} \, W(J_\Phi) \left[\left(2 - \frac{3\eta}{2}\right) F(\beta(l)) + (4-\eta)\beta(l) \, F'(\beta(l)) + \beta(l)^2 \, F''(\beta(l))\right].
\end{aligned}
\tag{H.41}
$$

Following the finite temperature RG scheme [14], $\frac{\Delta C_V^{(1)}}{T}$ is evaluated at the value of $l = l_0$ at which $m_\Phi(l_0)$ is renormalized to of order of one, i.e. $m_\Phi(l_0) \approx \mathcal{O}(1)$ as mentioned previously. Substituting $T/T_{LFL}$ for $T(l_0)$, we arrive

$$
\Delta\gamma^{(1)}(T/T_{LFL}) = -\frac{1}{4} u_\Phi \left(\frac{T_{LFL}}{T}\right)^{3-\frac{\eta}{2}} \left[\left(2 - \frac{3\eta}{2}\right) F(\beta) + (4-\eta)\beta \, F'(\beta) + \beta^2 \, F''(\beta)\right] \Big|_{\beta = \frac{T_{LFL}}{T}},
\tag{H.42}
$$

where

$$
F\left(\beta \to \frac{T_{LFL}}{T}\right) = \int_{m_\Phi/T}^{m_\Phi \Lambda/T} \frac{dx}{x^{2-\eta/2}} \left[\frac{4}{(e^x-1)^2} + \frac{4}{e^x - 1} + 1\right].
\tag{H.43}
$$

Here, we define the leading correction to normalized specific heat coefficient as

$$
\Delta\gamma^{(1)}(T/T_{LFL}) = \frac{\Delta C_V^{(1)}}{A'(l_0) T}
\tag{H.44}
$$

with the scaling dependent prefactor $A'(l_0) \equiv e^{z(3-\eta/2)l_0} \, W(J_\Phi)$. Including the contributions from the quartic term in $u_\Phi$, the result is shown in Fig. 7 where a negligible correction to $\gamma(T/T_{LFL})$ is found (except at very low temperatures where $T/T_{LFL} \ll 1$). Thus, $\Delta^{(1)}\gamma(T/T_{LFL})$ does not affect the power-law scaling behaviors for $\gamma(T/T_{LFL})$ in the scaling regime.

### H.2. Resistivity

To obtain the electrical resistivity as a function of temperature $\rho(T)$, we first calculate the scattering rate $\tau^{-1}(\omega)$ of itinerant electrons and the $T$-matrix $T_{\mathbf{kk}}(\omega)$, given by [17]

$$
\tau^{-1}(\omega) = -2 \sum_{\mathbf{k}} \mathrm{Im}\Sigma_c(\omega^+, \mathbf{k}) \;, \quad \Sigma_c(\omega^+, \mathbf{k}) = c_{imp} \, T_{\mathbf{kk}}(\omega^+).
\tag{H.45}
$$

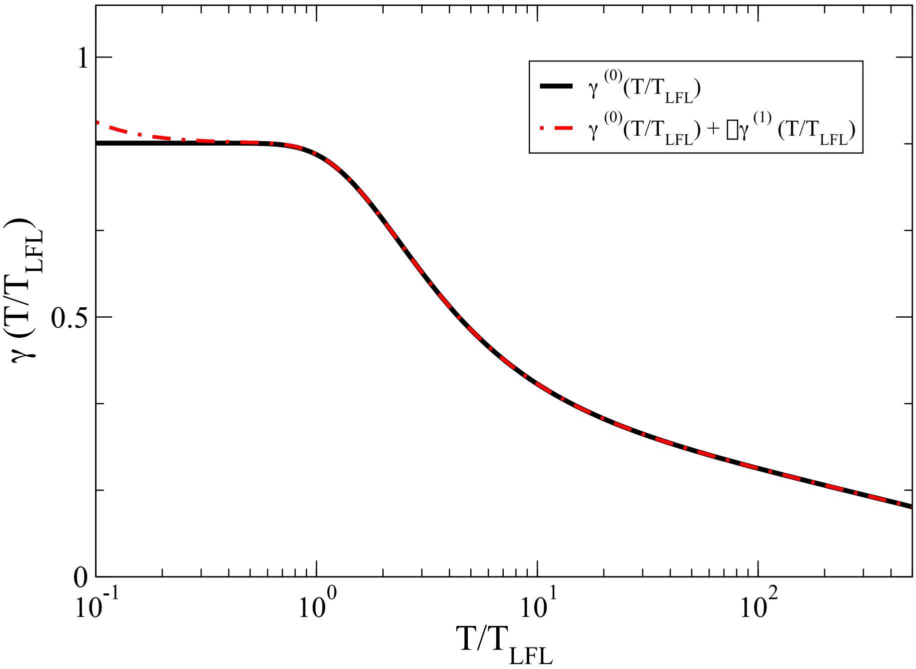


FIG. 7: The curve in red double-dotted dashed line represents the specific heat coefficient at $J_\Phi - J_\Phi^* = 0.4$ by including the contribution from the quartic term with the bare value of $u_\Phi$ being $u_\Phi/D_0 = 10^{-5}$. This shows that the first-order correction $\Delta^{(1)}\gamma(T/T_{LFL})$ in $u_\Phi$ to $\gamma(T/T_{LFL})$ is negligibly small.

where $\Sigma_c$ denotes the self-energy of itinerant electrons :

$$\begin{aligned}\Sigma_c(i\omega) =& \frac{2J_\chi^2}{\beta}\sum_{i\nu,\,\mathbf{k}} G_f^b(i\nu)G_\chi^b(i\omega - i\nu)\\ =& \frac{2J_\chi^2}{\beta}\sum_{i\nu,\,\mathbf{k}}\left[\frac{1}{i\nu - i\omega - \epsilon_\chi(\mathbf{k})} - \frac{1}{i\nu - i\omega - \epsilon_\chi(\mathbf{k})}\right]\frac{1}{i\nu - \bar{\lambda} - \Sigma_f^{(2)}(i\nu)},\end{aligned} \tag{H.46}$$

where, in the wideband limit, $\Sigma_f^{(2)}(i\omega) = i\,\mathrm{sgn}(\omega)\Gamma$ with $\Gamma = -2\pi J_\chi^2 N_0$. Note that the leading contributions to $T_{\mathbf{kk}}(\omega)$ (or equivalently the imaginary part of $\Sigma_c$) come from the quantum fluctuation of $\hat{\tilde{\chi}}_k$. Here, we only consider the temperature higher than $T^*$; thus due to the thermal fluctuation, the mass of the $\hat{\tilde{\chi}}$-field, $m'_\chi$, is neglected in the bare Green's function of the $\hat{\tilde{\chi}}$-field throughout the calculation of resistivity.

Due to the sign function $\mathrm{sgn}(\omega)$ in $\Sigma_f^{(2)}(i\omega)$, the Matsubara sum for the $c$-electron self-

energy $\Sigma_c(i\omega)$ in Eq. (H.46) should be performed for $\nu > 0$ and $\nu < 0$ cases separately, leading to the following expression for $\Sigma_c(i\omega)$

$$\Sigma_c(i\omega) \equiv f_+(\omega) + f_-(\omega), \tag{H.47}$$

where $f_{+(-)}(\omega)$ refers to the results after Matsubara sum for $\nu > 0 (< 0)$, respectively. The $f_+(\omega)$ is obtained by a contour integral over the upper complex $z$-plane upon the generalization $i\nu \to z$, given by:

$$\begin{aligned} f_+(\omega) =& 2J_\chi^2 \sum_{\mathbf{k}} \left[ \frac{n_F(\bar{\lambda} + i\Gamma)}{-i\omega + \bar{\lambda} + i\Gamma - \epsilon_\chi(\mathbf{k})} - \frac{n_F(\bar{\lambda} + i\Gamma)}{-i\omega + \bar{\lambda} + i\Gamma + \epsilon_\chi(\mathbf{k})} \right. \\ & \left. + \frac{n_F(i\omega + \epsilon_\chi(\mathbf{k}))}{i\omega + \epsilon_\chi(\mathbf{k}) - \bar{\lambda} - i\Gamma} - \frac{n_F(i\omega - \epsilon_\chi(\mathbf{k}))}{i\omega - \epsilon_\chi(\mathbf{k}) - \bar{\lambda} - i\Gamma} \right] \\ =& -2J_\chi^2 \sum_{\mathbf{k}} \frac{1}{i\omega + \epsilon_\chi(\mathbf{k}) - \bar{\lambda} - i\Gamma}. \end{aligned} \tag{H.48}$$

Similarly, $f_-(\omega)$ is given by:

$$f_-(\omega) \; = \; 2J_\chi^2 \sum_{\mathbf{k}} \frac{1}{i\omega + \epsilon_\chi(\mathbf{k}) - \bar{\lambda} + i\Gamma}. \tag{H.49}$$

Upon analytic continuation, $i\omega \to \omega + i\delta$ with $\omega > 0$ (relative to the Fermi energy $\epsilon_F$), the imaginary part of $\Sigma_c(\omega)$ becomes

$$\operatorname{Im}\Sigma_c(\omega) = -4J_\chi^2 N_0 \Gamma \int_0^\Lambda \frac{d\epsilon}{(\omega+\epsilon)^2 + \Gamma^2} + \mathcal{O}(\eta) \;\; = -4J_\chi^2 N_0 \Gamma \left[ \tan^{-1}\left(\frac{\Lambda + \omega}{\Gamma}\right) - \tan^{-1}\frac{\omega}{\Gamma} \right]. \tag{H.50}$$

Here, $\omega$ is shifted by $\bar{\lambda}$: $\omega \to \omega - \bar{\lambda}$, and we neglect the higher order terms in $\eta$. Eq. (H.50) can be further simplified as

$$\tan^{-1}\left(\frac{\Lambda+\omega}{\Gamma}\right) = \theta + \delta\theta, \quad \text{for } \theta \gg \delta\theta. \tag{H.51}$$

We assume that $\Lambda \gg \omega$, $\Gamma$ and $\Gamma \gg \omega$. Let us define $D \equiv \Lambda/\Gamma$ and $\delta D \equiv \omega/\Gamma$, we therefore have

$$\tan(\theta + \delta\theta) = D + \delta D \approx \tan\theta + \delta\theta \sec^2\theta \Rightarrow \; \delta\theta = \frac{\omega}{\Gamma}\cos^2\left(\tan^{-1}\frac{\Lambda}{\Gamma}\right).$$

Similarly, for $\Gamma \gg \omega$, we have (see Eq. (H.50))

$$\tan^{-1}\frac{\omega}{\Gamma} \approx \frac{\omega}{\Gamma}. \tag{H.52}$$

Finally, we find that the imaginary part of itinerant-electron self-energy $\mathrm{Im}\,\Sigma_c(\omega^+)$ is linearly proportional to $\omega$:

$$\begin{aligned}\mathrm{Im}\ \Sigma_c(\omega > 0) \approx &- 4J_\chi^2 N_0 \Gamma \left[\tan^{-1}\frac{\Lambda}{\Gamma} + \frac{\omega}{\Gamma}\left(\cos^2\left(\tan^{-1}\frac{\Lambda}{\Gamma}\right) - 1\right)\right] \\ \equiv &- (\alpha - \gamma\omega). \end{aligned} \tag{H.53}$$

where $\alpha = -4J_\chi^2 N_0 \Gamma \tan^{-1}\frac{\Lambda}{\Gamma} \approx -2\pi J_\chi^2 N_0 \Gamma$, $\gamma = 4J_\chi^2 N_0 \cos^2\left(\tan^{-1}\frac{\Lambda}{\Gamma} - 1\right) \approx -4N_0 J_\chi^2$.

For $\omega < 0$, the calculations for $\Sigma_c$ are the same as that for $\omega > 0$ except for $\omega \to -\omega$ and $\nu \to -\nu$, leading to $\mathrm{Im}\ \Sigma(\omega < 0) = -(\alpha + \gamma\omega)$. Therefore, we have

$$\mathrm{Im}\ \Sigma(\omega) = -(\alpha - \gamma|\omega - \epsilon_F|). \tag{H.54}$$

Combining Eq. (H.45) and Eq. (H.54), for an isotropic system, the conductivity is then given by [17]

$$\begin{aligned}\sigma(T) &= -\frac{2e^2}{3}\int \frac{d\mathbf{k}}{(2\pi)^3} v_k^2 \tau(k) \frac{\partial f}{\partial \epsilon_k} = -\frac{2e^2}{3}\int k^{\eta+1} dk \frac{k^2}{m^2}\tau(k)\frac{\partial f}{\partial \epsilon_k} \\ &= \frac{2e^2}{3}\int_{-\infty}^{\infty} \omega^{1+\eta/2}\left(\alpha - \gamma|\omega|\right)^{-1}\frac{\partial f(\omega - \epsilon_F)}{\partial \omega} d\omega \\ &\approx \frac{2e^2|\epsilon_F|^{1+\eta/2}}{3|\alpha|}\int_{-\infty}^{\infty}(-1 + \frac{\gamma}{|\alpha|}|\omega - \epsilon_F|)\frac{\partial f(\omega - \epsilon_F)}{\partial \omega} d\omega \\ &= a + bT\int_{-\infty}^{\infty}|x|\frac{\partial f}{\partial x}dx \\ &= a - cT \end{aligned} \tag{H.55}$$

with $x = (\omega - \epsilon_F)/T$, and $a$, $b$, $c$ being constant pre-factors, while the integral $\int_{-\infty}^{\infty}|x|(\partial f/\partial x)dx \approx -1.386$, $a = 2\,e^2\,\epsilon_F^{1+\eta/2}/(3|\alpha|)$, $c = 1.386\,a\,\gamma/|\alpha|$ and the ratio $\gamma/|\alpha| = 2/\pi\Gamma = 1/\pi^2 J_\chi^2 N_0$. Therefore, the resistivity $\rho(T)$ is given by

$$\rho(T) = \frac{1}{\sigma(T)} \approx \frac{1}{a}\left(1 + \frac{c}{a}T\right). \tag{H.56}$$

Therefore, $\Delta\rho/\rho_0 = c\,\Delta T/a = 1.386\,\Delta T/(\pi^2 J_\chi^2 N_0) \approx 1.76$ with $\Delta T = 0.9\,K$ and $J_\chi^2 N_0/4 \equiv T_{\mathrm{Neel}} = 18\,\mathrm{mK}$ for Ge-substituted $\mathrm{YbRh_2Si_2}$. Our result for $\Delta\rho/\rho_0$ is in reasonable agreement with the experimental value $\Delta\rho/\rho_0 \approx 0.44$ for $\Delta T = 0.9$ [12, 18, 19].

### H.3. Local spin susceptibility $\chi_{loc}(T)$

At zero magnetic field and high temperature regime ($T \gg T^*$), we can simply estimate the anomalous exponent $\eta_\chi$ for the local spin susceptibility $\chi_{loc}(T)$ via the bare scaling

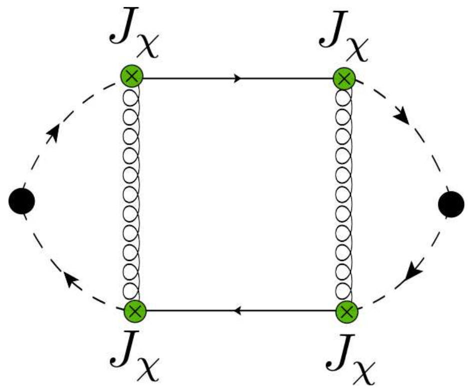


FIG. 8: The Feynman diagram to the 4$^{\text{th}}$ order in $J_\chi$ for the local susceptibility $\chi_{\text{loc}}(T)$. Here, the filled $\otimes$ symbols represent the interaction vertices for $J_\chi$.

dimension of the lowest non-trivial order diagram in Fig. 8:

$$\chi_{loc}(T) \propto \frac{J_\chi^4}{T} \propto T^{2\eta-1} = T^{-0.75}, \tag{H.57}$$

where the bare scaling for $[J_\chi] = \eta/2$ (or $J_\chi(T) \sim T^{-\eta/2}$) is used. Experimentally, $\chi_{loc}(T) \sim T^{-p}$ with $p \approx 0.75$ [11, 19]. When taking the optimized value of $\eta \sim 0.18$ fitted to the normalized specific heat coefficient $\gamma(T/T_{LFL})$, here, we get $\chi_{loc}(T) \sim T^{2\eta-1} \sim T^{-\bar{p}}$ with $\bar{p} \approx 0.64$, in reasonable agreement with the experimental value shown above [11, 19].

## I. FERMI SURFACE JUMP AND THE $\frac{\omega}{T}$ SCALING

In this section, we discuss issue the Fermi surface jump when the parameter $g$ is tuned across $g_c$ at zero temperature. We shall prove that at $g > g_c$ the Fermi surface is enlarged due to the existence of Kondo hybridization via the Anderson model. Next, we address the issue of the $\omega/T$ scaling at finite temperature $T > 0$.

### I.1. Fermi surface jump

To start with, we consider the Anderson Hamiltonian, given by

$$H = \sum_{\mathbf{k}\sigma} \epsilon_c(\mathbf{k}) c^\dagger_{\mathbf{k}\sigma} c_{\mathbf{k}\sigma} + \sum_{\mathbf{k}\sigma} \bar{\lambda} f^\dagger_{\mathbf{k}\sigma} f_{\mathbf{k}\sigma} + \sum_{\mathbf{k}\sigma} \left( \chi_{\mathbf{k}} c^\dagger_{\mathbf{k}\sigma} f_{\mathbf{k}\sigma} + h.c. \right). \tag{I.1}$$

where we denote $\epsilon_c(\mathbf{k})$ as the dispersion relative to the chemical potential for the conduction electrons $c_{\mathbf{k}}$, $\sigma = \uparrow, \downarrow$ as the spin indices and $\chi_{\mathbf{k}}$ as the mean-field value for the Kondo

correlation. As Kondo effect takes place, we anticipate a change in the dispersion for $c$-electrons. To this end, we compute the self-energy $\Sigma_c$ for the conduction electrons at the mean-field level at zero temperature and see what happens to the dispersion for $c$-electrons via Kondo effect. From perturbation theory, $\Sigma_c$ can be obtained

$$\Sigma_c(\mathbf{k}, i\omega) = \frac{|\chi|^2}{i\omega - \bar{\lambda}} \;\Rightarrow\; \Sigma_c(\mathbf{k}, \omega + i\delta) = \frac{|\chi|^2}{\omega - \bar{\lambda}} - i\pi\delta(\omega - \bar{\lambda}) = \frac{|\chi|^2}{\omega - \bar{\lambda}}. \tag{I.2}$$

Here, a $\mathbf{k}$-independent Kondo hybridization $\chi_{\mathbf{k}} = \chi$ is assumed. In Eq. (I.2), we analytically continue the Matsubara frequency to the real frequency. The Dirac $\delta(\omega - \bar{\lambda})$ function vanishes in Eq. (I.2) since $\lambda \gg \omega$, leading to a purely real self-energy $\Sigma_c$ at the mean-field level. A real self-energy $\Sigma_c$ also implies no Laudau damping, leading to a Fermi surface jump at zero temperature at QCP $g_c$.

For $g < g_c$, the mean-field value of $\chi$ vanishes since the local moments are decoupled with conduction electrons, leading to $\Sigma_c(\mathbf{k}, \omega) = 0$. The $c$-electron Green's function is simply given by $G_c(\mathbf{k}, \omega + i\delta) = (\omega - \epsilon_c(\mathbf{k}))^{-1}$. At $\mathbf{k} = k_F$ (or $\epsilon_c(\mathbf{k}_F) = 0$), a pole occurs at $\omega = 0$. As $g$ exceeds $g_c$, the hybridization of the local moments and the conduction electrons develops and the system enters the Kondo regime with finite $\chi$. The renormalized Green function for the conduction electrons then becomes

$$G_c(\mathbf{k}, \omega + i\delta) = \frac{1}{\omega - \epsilon_c(\mathbf{k}) - |\chi|^2/(\omega - \bar{\lambda})}. \tag{I.3}$$

At $\mathbf{k} = k_F$, $\omega = 0$ is no longer a pole for $G_c$ in Eq. (I.3), which signifies that $k_F$ is not the Fermi momentum when the hybridization occurs. The new Fermi momentum $k_F^*$ at $g > g_c$ can be determined via the similar way: finding a certain value $\mathbf{k} = k_F^*$ at which a pole develops at $\omega = 0$ in Eq. (I.3). At $\omega = 0$, the Green's function in Eq. (I.3) becomes

$$G_c(\mathbf{k}, \omega = 0) = \frac{\bar{\lambda}}{|\chi|^2 - \bar{\lambda}\,\epsilon_{\mathbf{k}}}. \tag{I.4}$$

Eq. (I.4) diverges at $\epsilon_c(\mathbf{k}) \equiv \frac{\mathbf{k}^2}{2m} - \epsilon_F = |\chi|^2/\bar{\lambda}$. The new Fermi energy $\epsilon_F^*$ is given by

$$\epsilon_F^* = \frac{k_F^{*2}}{2m} \equiv \epsilon_F + \frac{|\chi|^2}{\bar{\lambda}}. \tag{I.5}$$

Thus, as the parameter $g$ is tuned to $g_c^+$, the Fermi energy enlarges by a small amount of value $|\chi|^2/\bar{\lambda}$ due to the mean-field Kondo hybridization, which signifies only a small fraction of local $f$-electrons participate in the formation of the new Fermi surface at $g > g_c$. Together with the result of the real self-energy for the conduction electrons in Eq. (I.2), the

Fermi surface will evolve discontinuously across $g_c$, in well agreement with the experimental findings.

Besides, the quasiparticle weight factor $Z$, defined as

$$Z = \left(1 - \frac{\partial \mathrm{Re}\,\Sigma_c}{\partial \omega}\right)^{-1}, \tag{I.6}$$

vanishes at $\omega = 0$. The proof is quite straightforward: via Eq. (I.2), the derivative of real part self-energy is given by

$$\frac{\partial \mathrm{Re}\Sigma_c}{\partial \omega} = -\frac{|\chi|^2}{(\omega - \bar{\lambda})^2} = -\frac{|\chi|^2}{\omega^2}. \tag{I.7}$$

In the second line of the above equation, we shift the frequency by the constant $\bar{\lambda}$. At $\omega = 0$, $\partial \mathrm{Re}\Sigma_c/\partial\omega$ diverges, leading to $Z \to 0$. The divergence of $\partial \mathrm{Re}\Sigma_c/\partial\omega$ at $\omega = 0$ also gives rise to the divergence of the renormalized mass, which is given by $m^*/m \propto 1 - \frac{\partial \mathrm{Re}\,\Sigma_c}{\partial \omega}$ with $m^*$ being the renormalized mass and $m$ being the bare mass.

### I.2. $\omega/T$ scaling of the Hall crossover

In experiments, a linear-$T$ dependence of the fullwidth half-magnitude (FWHM) of the Hall crossover, which measures the broadening of the conduction electron spectral weight, at the crossover regime has been observed [7], implying a linear-$T$ dependence of the imaginary part of the self-energy $\Sigma_c$ of the conduction electrons and giving a solid evidence of the dynamical scaling behavior at finite temperature. In the following, we shall show that the imaginary part of the conduction electron self-energy in our theory indeed linearly depends on temperature.

The self-energy of the conduction electron $\Sigma_c$ contributed from the fluctuation of the Kondo hybridization has been shown in Eq. (H.46) while self-energy $\Sigma_f^{(2)}(i\omega)$ of the local $f$-electrons in Eq. (H.46) is expressed as

$$\Sigma_f^{(2)}(i\omega) = 2J_\chi^2 \sum_{\mathbf{k}} \left[\frac{1 + n_B(\epsilon_\chi(\mathbf{k}))}{\omega - \epsilon_c(\mathbf{k}) - \epsilon_\chi(\mathbf{k})} - \frac{-n_B(\epsilon_\chi(\mathbf{k}))}{\omega - \epsilon_c(\mathbf{k}) + \epsilon_\chi(\mathbf{k})}\right]. \tag{I.8}$$

In order to obtain a temperature-dependent imaginary part of the conduction electron self-energy $\Sigma_c$, we expand the Bose function $n_B$ in $\Sigma_f^{(2)}$ to the first order in $T$ via assuming $\beta\epsilon_\chi(\mathbf{k}) \ll 1$ (or $T \gg \epsilon_\chi(\mathbf{k})$). We get the approximate Bose function $n_B(\epsilon_\chi(\mathbf{k})) \approx 1/\beta\epsilon_\chi(\mathbf{k}) =$

$T/\epsilon_\chi(\mathbf{k})$. Taking the approximation $\epsilon_c(\mathbf{k}) \gg \epsilon_\chi(\mathbf{k})$, Eq. (I.8) becomes

$$\Sigma_f^{(2)}(i\omega) = 2J_\chi^2 \sum_{\mathbf{k}} \left[\frac{1}{i\omega - \epsilon_c(\mathbf{k})}\right] + 4J_\chi^2 T \sum_{\mathbf{k}} \left(\frac{1}{\epsilon_\chi(\mathbf{k})} \cdot \frac{1}{i\omega - \epsilon_c(\mathbf{k})}\right). \tag{I.9}$$

The $T$-independent term in Eq. (I.9) has been already derived in the wideband limit, which is given by $-i\,\mathrm{sgn}(\omega)\Gamma$ with $\Gamma \equiv 2\pi N_0 J_\chi^2$.

To analyze the $T$-dependent term in Eq. (I.9), it is convenient to rewrite the dispersion $\epsilon_\chi(\mathbf{k})$ as

$$\epsilon_\chi(\mathbf{k}) = \begin{cases} 0, \;\; \text{if} \;\; -\Lambda < \epsilon_c(\mathbf{k}) < 0 \\ \\ a\epsilon_c(\mathbf{k}), \;\text{if} \;\; 0 < \epsilon_c(\mathbf{k}) < \Lambda \end{cases} = a\epsilon_c(\mathbf{k})\Theta(\epsilon_c(\mathbf{k})). \tag{I.10}$$

Here, the constant prefactor $a = N_0 J_\chi^2/\bar{\lambda}$. The $T$-linear term in Eq. (I.9) is then given by

$$\begin{aligned} &\frac{4J_\chi^2 T}{a} \sum_{\mathbf{k}} \frac{1}{a\epsilon_c(\mathbf{k})\Theta(\epsilon_c(\mathbf{k}))\,[i\omega - \epsilon_c(\mathbf{k})]} = \frac{4J_\chi^2 N_0 T}{a} \int_\zeta^\Lambda d\epsilon_c \left(\frac{1}{\epsilon_c} + \frac{1}{i\omega - \epsilon_c}\right) \\ =&\frac{4J_\chi^2 N_0 T}{ia\omega}\left[\ln\frac{\Lambda}{\zeta} - \ln\left(\frac{i\omega - \Lambda}{i\omega + \zeta}\right)\right], \end{aligned} \tag{I.11}$$

where $\ln\left(\frac{i\omega-\Lambda}{i\omega+\zeta}\right) \approx \ln(\Lambda/\sqrt{2}\zeta) + i\mathrm{sgn}(\omega)\pi/4$ in the regime $\omega \sim \zeta$. Note that we have introduced a lower energy cutoff $\zeta \propto (L)^{-2}$, which is inversely proportional the square of the length $L$ of the system size in the above integral to avoid the infra-red divergence. The $T$-dependent term in $\Sigma_f^{(2)}$ in Eq. (I.11) becomes

$$\frac{\kappa}{i\omega}\left(\ln\sqrt{2} - i\mathrm{sgn}(\omega)\frac{\pi}{4}\right). \tag{I.12}$$

with $\kappa \equiv 4J_\chi^2 T N_0/a = 4\bar{\lambda}T$ being a $T$-dependent prefactor.

Combining Eq. (H.46) and Eq. (I.12), the self-energy $\Sigma_f^{(2)}(i\omega)$ of the local $f$-electrons contributed from the fluctuation of the Kondo hybridization is then given by

$$\Sigma_f^{(2)}(i\omega) = -i\mathrm{sgn}(\omega)\Gamma + \frac{\kappa}{i\omega}\left(\ln\sqrt{2} - i\mathrm{sgn}(\omega)\frac{\pi}{4}\right). \tag{I.13}$$

Via Eq. (I.13), the self-energy for the $c$-electron in Eq. (H.46) is then given by

$$\begin{aligned}\Sigma_c(i\omega,\,\mathbf{k}) &= \frac{2J_\chi^2}{\beta}\sum_{i\nu}\left[\frac{1}{i\nu - i\omega - \epsilon_\chi(\mathbf{k})} - \frac{1}{i\nu - i\omega + \epsilon_\chi(\mathbf{k})}\right] \\ &\qquad\times\frac{1}{i\nu - \bar{\lambda} + i\mathrm{sgn}(\nu)\Gamma - \frac{\kappa}{i\nu}\left(\ln\sqrt{2} - i\mathrm{sgn}(\nu)\frac{\pi}{4}\right)} \\ &= \frac{2J_\chi^2}{\beta}\sum_{i\nu}\left[\frac{1}{i\nu - i\omega - \epsilon_\chi(\mathbf{k})} - \frac{1}{i\nu - i\omega + \epsilon_\chi(\mathbf{k})}\right] \\ &\qquad\times\frac{1}{2\alpha_2}\left[\frac{\alpha_1+\alpha_2}{i\nu - (\alpha_1+\alpha_2)} - \frac{\alpha_1-\alpha_2}{i\nu-(\alpha_1-\alpha_2)}\right].\end{aligned} \tag{I.14}$$

where $\alpha_1 \equiv (\bar{\lambda} - i\Gamma\,\mathrm{sgn}(\nu)\,)/2$ and $\alpha_2 \equiv (\bar{\lambda} - i\Gamma\,\mathrm{sgn}(\nu)\,)/2 + 4T\ln\sqrt{2} - i\pi T\,\mathrm{sgn}(\nu)$. It is clear that due the function $\mathrm{sgn}(\nu)$ the poles in Eq. (I.14) depend on the sign of the Matsubara frequency $\nu$, signifying that we must evaluate the Matsubara sum for the positive frequencies $\nu > 0$ and the negative frequencies $\nu < 0$ separately.

### *1. For* $\nu > 0$

For $\nu > 0$, the poles in the term contributed from $\Sigma_f^{(2)}$ in Eq. (I.14) are given by

$$\alpha_1 + \alpha_2 \equiv \bar{\lambda} - i\Gamma - i\pi T \quad ; \quad \alpha_1 - \alpha_2 \equiv -4T\ln\sqrt{2} + i\pi T. \tag{I.15}$$

Via Eq. (I.15), $\Sigma_c$ takes the form

$$\begin{aligned}\Sigma_c(\mathbf{k}, i\omega) = \frac{2J_\chi^2}{\bar{\lambda} - i\Gamma - 2\pi i T}\cdot\frac{1}{\beta}\sum_{\nu>0}\left[\frac{1}{i\nu - i\omega - \epsilon_\chi(\mathbf{k})} - \frac{1}{i\nu - i\omega + \epsilon_\chi(\mathbf{k})}\right] \\ \times\left[\frac{\bar{\lambda} - i\Gamma - i\pi T}{i\nu - \bar{\lambda} + i\Gamma + i\pi T} - \frac{-4T\ln\sqrt{2} + i\pi T}{i\nu + 4T\ln\sqrt{2} - i\pi T}\right]\end{aligned} \tag{I.16}$$

The direct approach to perform the Matsubara sum in Eq. (I.16) over the positive fermionic Matsubara frequencies $\nu = \pi(2n+1)/\beta$ with $n = 0, 1, 2\cdots$ is to introduce a contour integral with poles occur at $i\nu$'s, given by

$$\begin{aligned}I_+(i\omega, \mathbf{k}) \equiv \oint_{\mathbb{C}}\frac{dz}{2\pi i}\,n_F(z)\left[\frac{1}{z - i\omega - \epsilon_\chi(\mathbf{k})} - \frac{1}{z - i\omega + \epsilon_\chi(\mathbf{k})}\right] \\ \times\left[\frac{\bar{\lambda} - i\Gamma - i\pi T}{z - \bar{\lambda} + i\Gamma + i\pi T} - \frac{-4T\ln\sqrt{2} + i\pi T}{z + 4T\ln\sqrt{2} - i\pi T}\right]\end{aligned} \tag{I.17}$$

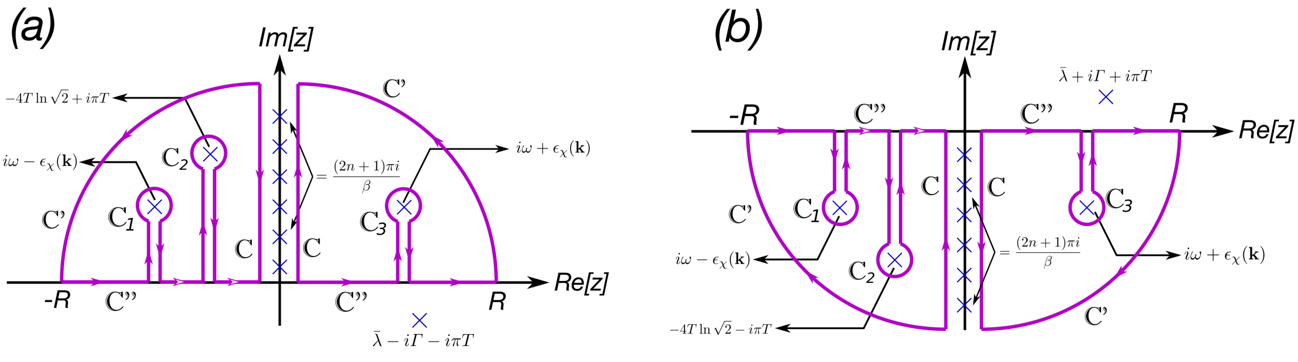


FIG. 9: Figures (a) and (b) schematically show the contours chosen on the complex $z$-plane to evaluate the Matsubara sum for the case of $\nu > 0$ and $\nu < 0$, respectively. $R$ denotes the radius of the contours. The poles are represented by the cross symbols "×".

The contour $\mathbb{C}$ for $I_+$ in Eq. (I.17) is chosen to counterclockwise circle around the complex axis in the $z$-plane as shown in Fig. 9-(a). Inside the contour $\mathbb{C}$, the singularities are simple poles at $i\nu$'s and Cauchy's residue theorem yields

$$I_+(i\omega,\,\mathbf{k}) = -\frac{1}{\beta}\sum_{\nu>0}\left[\frac{1}{i\nu - i\omega - \epsilon_\chi(\mathbf{k})} - \frac{1}{i\nu - i\omega + \epsilon_\chi(\mathbf{k})}\right] \times \left[\frac{\bar\lambda - i\Gamma - i\pi T}{i\nu - \bar\lambda + i\Gamma + i\pi T} - \frac{-4T\ln\sqrt{2} + i\pi T}{i\nu + 4T\ln\sqrt{2} - i\pi T}\right] \tag{I.18}$$

The standard technique for the Matsubara sum then requires to deform the contour $\mathbb{C}$ into $\mathbb{C}_1$, $\mathbb{C}_2$, $\mathbb{C}_3$, $\mathbb{C}'$ and $\mathbb{C}''$ as illustrated in Fig. 9-(a), where $\mathbb{C}''$ is along the real axis. Integrating along the semicircle $\mathbb{C}'$ vanishes as the radius $R$ of $\mathbb{C}'$ approaches to infinity. Only the integration along $\mathbb{C}_1$, $\mathbb{C}_2$, $\mathbb{C}_3$ and $\mathbb{C}''$ survives, leading to

$$\begin{aligned}
&I_+(i\omega,\,\mathbf{k}) \\
=\;& -\Theta(\omega)n_F(i\omega+\epsilon_\chi(\mathbf{k}))\left[\frac{\bar\lambda - i\Gamma - i\pi T}{i\omega+\epsilon_\chi(\mathbf{k}) - \bar\lambda + i\Gamma + i\pi T} - \frac{-4T\,\ln\sqrt{2}+i\pi T}{i\omega+\epsilon_\chi(\mathbf{k}) + 4T\,\ln\sqrt{2} - i\pi T}\right] \\
&+\Theta(\omega)n_F(i\omega-\epsilon_\chi(\mathbf{k}))\left[\frac{\bar\lambda - i\Gamma - i\pi T}{i\omega-\epsilon_\chi(\mathbf{k}) - \bar\lambda + i\Gamma + i\pi T} - \frac{-4T\,\ln\sqrt{2}+i\pi T}{i\omega-\epsilon_\chi(\mathbf{k}) + 4T\,\ln\sqrt{2} - i\pi T}\right] \\
&+n_F(-4T\,\ln\sqrt{2}+i\pi T)\left[\frac{-4T\,\ln\sqrt{2}+i\pi T}{-i\omega-\epsilon_\chi(\mathbf{k}) - 4T\,\ln\sqrt{2}+i\pi T}\right. \\
&\qquad\left. - \frac{-4T\,\ln\sqrt{2}+i\pi T}{-i\omega+\epsilon_\chi(\mathbf{k}) - 4T\,\ln\sqrt{2}+i\pi T}\right] \\
&+J_+(i\omega,\,\mathbf{k}),
\end{aligned} \tag{I.19}$$

where $J_+(\omega)$ is an integral along the real axis $\mathbb{C}''$, given by

$$\begin{aligned} J_+(i\omega,\, \mathbf{k}) \;&= \int_{-\infty}^{\infty} \frac{dy}{2\pi i}\, n_F(y) \qquad \left[\frac{1}{y - i\omega - \epsilon_\chi(\mathbf{k})} - \frac{1}{y - i\omega + \epsilon_\chi(\mathbf{k})}\right] \\ &\qquad\qquad\qquad\qquad \times \left[\frac{\bar{\lambda} - i\Gamma - i\pi T}{y - \bar{\lambda} + i\Gamma + i\pi T} - \frac{-4T \ln\sqrt{2} + i\pi T}{y + 4T\ln\sqrt{2} - i\pi T}\right] \\ &= \int_{-\infty}^{0} \frac{dy}{2\pi i} \left[\frac{1}{y - i\omega - \epsilon_\chi(\mathbf{k})} - \frac{1}{y - i\omega + \epsilon_\chi(\mathbf{k})}\right] \\ &\qquad\qquad\qquad\qquad \times \left[\frac{\bar{\lambda} - i\Gamma - i\pi T}{y - \bar{\lambda} + i\Gamma + i\pi T} - \frac{-4T \ln\sqrt{2} + i\pi T}{y + 4T\ln\sqrt{2} - i\pi T}\right]. \end{aligned} \tag{I.20}$$

Applying the assumptions $\bar{\lambda} \gg T \gg \epsilon_\chi(\mathbf{k})$ in Eq. (I.19) and analytically continuing the Matsubara frequency to the real frequency space $i\omega \to \omega + i\delta$, $\Sigma_c$ for the situation of $\nu > 0$ is expressed as

$$\begin{aligned} &\Sigma_c(\omega + i\delta,\, \mathbf{k}) \\ &= -\frac{2J_\chi^2}{\bar{\lambda} - i\Gamma - 2\pi i T} \cdot \left\{ \Theta(\delta) \left[\frac{\bar{\lambda} - i\Gamma - i\pi T}{\omega - \epsilon_\chi(\mathbf{k}) - \bar{\lambda} + i\Gamma + i\pi T} - \frac{-4T\,\ln\sqrt{2} + i\pi T}{\omega - \epsilon_\chi(\mathbf{k}) + 4T\,\ln\sqrt{2} - i\pi T}\right] \right. \\ &\qquad\qquad \left. + J_+(\omega + i\delta,\, \mathbf{k}) \right\}. \end{aligned} \tag{I.21}$$

We then evaluate $\Sigma_c$ at the limit $\omega \to 0$ and $\mathbf{k} \to k_F^*$. Under the assumption $\bar{\lambda} \gg T \gg \epsilon_\chi(\mathbf{k})$, we quickly find $J_+(\omega \to 0) = 0$. Only the first term in Eq. (I.21) leaves, which survives only for positive $\delta$ due the unit-step function $\Theta(\delta)$. The positive $\delta$ on the other hand indicates the retarded Green's function. Finally, we find

$$\begin{aligned} \Sigma_c(\omega \to 0,\, k_F^*) \;&\approx\; -\frac{2J_\chi^2\,(\bar{\lambda} + i\Gamma + 2\pi i T)}{\bar{\lambda}^2} \quad \cdot \left[-\frac{\epsilon_\chi^*\,\left(\bar{\lambda} - i\Gamma - i\pi T\right)}{\bar{\lambda}^2}\right] \\ &= \frac{2J_\chi^2\,\epsilon_\chi^*}{\bar{\lambda}^2}\left[1 + \left(\frac{\Gamma}{\bar{\lambda}}\right)^2 + 3\pi\,\left(\frac{T\Gamma}{\bar{\lambda}^2}\right) + 2\pi^2\left(\frac{T}{\bar{\lambda}}\right)^2\right] + i\,\frac{2\pi\,J_\chi^2\,\epsilon_\chi^*}{\bar{\lambda}^3}\,T, \end{aligned} \tag{I.22}$$

where we define $\epsilon_\chi^* \equiv \epsilon_\chi(k_F^*)$. Thus, the imaginary part of $\Sigma_c(\omega \to 0, k_F^*)$ for the case of $\nu > 0$ is given by

$$\mathrm{Im}\Sigma_c(\omega \to 0,\, k_F^*) = \frac{2\pi\,J_\chi^2\,\epsilon_\chi^*}{\bar{\lambda}^3}\,T. \tag{I.23}$$

It is clear that the imaginary part of $\Sigma_c$ in Eq. (I.23) contributed from summing over the positive Matsubara frequency $\nu$'s exhibits a linear-$T$ dependence, giving rise to a linear-in-$T$ broadening in the conduction-electron spectral weight [7].

*2. For $\nu < 0$*

For $\nu < 0$, the poles of the term contributed from $\Sigma_f^{(2)}$ in Eq. (I.14) are given by

$$\alpha_1 + \alpha_2 = \bar{\lambda} + i\Gamma + i\pi T \;\; ; \;\; \alpha_1 - \alpha_2 = -4T \ln\sqrt{2} - i\pi T. \tag{I.24}$$

Via Eq. (I.24), $\Sigma_c$ takes the form

$$\begin{aligned}\Sigma_c(\mathbf{k}, i\omega) = -\frac{2J_\chi^2}{\bar{\lambda} + i\Gamma + 2\pi i T} \cdot \frac{1}{\beta} \sum_{\nu<0} &\left[\frac{1}{i\nu - i\omega - \epsilon_\chi(\mathbf{k})} - \frac{1}{i\nu - i\omega + \epsilon_\chi(\mathbf{k})}\right] \\ \times &\left[\frac{\bar{\lambda} + i\Gamma + i\pi T}{i\nu - \bar{\lambda} - i\Gamma - i\pi T} - \frac{-4T\ln\sqrt{2} - i\pi T}{i\nu + 4T\ln\sqrt{2} + i\pi T}\right]\end{aligned} \tag{I.25}$$

To perform the Matsubara sum over the negative Matsubara frequencies $\nu = (2n+1)\pi/\beta$ with $n \in -1, -2, \cdots$ in Eq. (I.25), we introduce the contour integral $I_-(\omega)$ with $\mathbb{C}$ being chosen to clockwise enclose the negative complex axis in the complex $z$-plane as shown in Fig. 9-(b), given by

$$\begin{aligned}I_-(i\omega, \mathbf{k}) \equiv \oint_{\mathbb{C}} \frac{dz}{2\pi i} n_F(z) &\left[\frac{1}{z - i\omega - \epsilon_\chi(\mathbf{k})} - \frac{1}{z - i\omega + \epsilon_\chi(\mathbf{k})}\right] \\ \times &\left[\frac{\bar{\lambda} + i\Gamma + i\pi T}{z - \bar{\lambda} - i\Gamma - i\pi T} - \frac{-4T\ln\sqrt{2} - i\pi T}{z + 4T\ln\sqrt{2} + i\pi T}\right].\end{aligned} \tag{I.26}$$

Via the Cauchy's residue integral, we reproduce the Matsubara sum over the negative $\nu$'s

$$\begin{aligned}I_-(i\omega, \mathbf{k}) = \frac{1}{\beta} \sum_{\nu<0} &\left[\frac{1}{i\nu - i\omega - \epsilon_\chi(\mathbf{k})} - \frac{1}{i\nu - i\omega + \epsilon_\chi(\mathbf{k})}\right] \\ \times &\left[\frac{\bar{\lambda} + i\Gamma + i\pi T}{i\nu - \bar{\lambda} - i\Gamma - i\pi T} - \frac{-4T\ln\sqrt{2} - i\pi T}{i\nu + 4T\ln\sqrt{2} + i\pi T}\right].\end{aligned} \tag{I.27}$$

Likewise, deform the contour $\mathbb{C}$ into $\mathbb{C}_1$, $\mathbb{C}_2$, $\mathbb{C}_3$, $\mathbb{C}'$ and $\mathbb{C}''$ as shown in Fig. 9-(b). It is clear that the integral along the lower semicircle $\mathbb{C}'$ in Eq. (I.26) vanishes as $R \to \infty$, only

the integral along $\mathbb{C}$ into $\mathbb{C}_1$, $\mathbb{C}_2$, $\mathbb{C}_3$ and $\mathbb{C}''$ leaves, giving rise to

$$
\begin{aligned}
& I_-(i\omega,\,\mathbf{k}) \\
= \;& \Theta(-\omega) n_F(i\omega + \epsilon_\chi(\mathbf{k})) \left[\frac{\bar{\lambda} + i\Gamma + i\pi T}{i\omega + \epsilon_\chi(\mathbf{k}) - \bar{\lambda} - i\Gamma - i\pi T} - \frac{-4T\,\ln\sqrt{2} - i\pi T}{i\omega + \epsilon_\chi(\mathbf{k}) + 4T\,\ln\sqrt{2} + i\pi T}\right] \\
& - \Theta(-\omega) n_F(i\omega - \epsilon_\chi(\mathbf{k})) \left[\frac{\bar{\lambda} + i\Gamma + i\pi T}{i\omega - \epsilon_\chi(\mathbf{k}) - \bar{\lambda} - i\Gamma - i\pi T} - \frac{-4T\,\ln\sqrt{2} - i\pi T}{i\omega - \epsilon_\chi(\mathbf{k}) + 4T\,\ln\sqrt{2} + i\pi T}\right] \\
& - n_F(-4T\,\ln\sqrt{2} - i\pi T) \left[\frac{-4T\,\ln\sqrt{2} - i\pi T}{-i\omega - \epsilon_\chi(\mathbf{k}) - 4T\,\ln\sqrt{2} - i\pi T}\right. \\
& \qquad \left. - \frac{-4T\,\ln\sqrt{2} - i\pi T}{-i\omega + \epsilon_\chi(\mathbf{k}) - 4T\,\ln\sqrt{2} - i\pi T}\right] \\
& + J_-(i\omega,\,\mathbf{k}),
\end{aligned}
\tag{I.28}
$$

where

$$
\begin{aligned}
J_-(i\omega,\,\mathbf{k}) \equiv & \int_{-\infty}^{\infty} \frac{dy}{2\pi i}\, n_F(y) \left[\frac{1}{y - i\omega - \epsilon_\chi(\mathbf{k})} - \frac{1}{y - i\omega + \epsilon_\chi(\mathbf{k})}\right] \\
& \times \left[\frac{\bar{\lambda} + i\Gamma + i\pi T}{y - \bar{\lambda} - i\Gamma - i\pi T} - \frac{-4T\ln\sqrt{2} - i\pi T}{y + 4T\ln\sqrt{2} + i\pi T}\right].
\end{aligned}
\tag{I.29}
$$

Following the similar approach, $\Sigma_c$ contributed from the negative Matsubara frequencies $\nu < 0$ takes the form

$$
\begin{aligned}
& \Sigma_c(\omega + i\delta,\,\mathbf{k}) \\
= \;& -\frac{2J_\chi^2}{\bar{\lambda} + i\Gamma + 2\pi i T} \cdot \left\{\Theta(-\delta) \left[\frac{\bar{\lambda} + i\Gamma + i\pi T}{\omega - \epsilon_\chi(\mathbf{k}) - \bar{\lambda} - i\Gamma - i\pi T} - \frac{-4T\,\ln\sqrt{2} - i\pi T}{\omega - \epsilon_\chi(\mathbf{k}) + 4T\,\ln\sqrt{2} + i\pi T}\right]\right. \\
& \qquad \left. - J_-(\omega + i\delta,\,\mathbf{k})\right\}.
\end{aligned}
\tag{I.30}
$$

For this case, we also find $J_-(\omega,\,\mathbf{k}) = 0$ at $\omega = 0$ under the assumption $\bar{\lambda} \gg T \gg \epsilon_\chi(\mathbf{k})$. In contrast to the previous case, $\Sigma_c$ survives only for negative $\delta$ due to the unit step function $\Theta(-\delta)$ in Eq. (I.30). The negative $\delta$ on the other hand implies advanced Green's function. Evaluating $\Sigma_c$ in Eq. (I.30) in the limit $\omega \to 0$ and $\mathbf{k} \to k_F^*$ yields

$$
\Sigma_c(\omega \to 0,\,k_F^*) = \frac{2J_\chi^2\,\epsilon_\chi^*}{\bar{\lambda}^2} \left[1 + \left(\frac{\Gamma}{\bar{\lambda}}\right)^2 + 3\pi\left(\frac{\Gamma T}{\bar{\lambda}^2}\right) + 2\pi^2\left(\frac{T}{\bar{\lambda}}\right)^2\right] - i\,\frac{2\pi J_\chi^2\,\epsilon_\chi^*}{\bar{\lambda}^3}\,T, \tag{I.31}
$$

where $\epsilon_\chi^* \equiv \epsilon_\chi(k_F^*)$. The imaginary part of $\Sigma_c(\omega \to 0,\, k_F^*)$ is then given by

$$\text{Im}\Sigma_c(\omega \to 0) = -\frac{2\pi J_\chi^2\, \epsilon_\chi^*}{\bar{\lambda}^3}\, T. \tag{I.32}$$

The imaginary part of $\Sigma_c$ in Eq. (I.32) also exhibits a linear-in-$T$ dependence. Here, we neglect this contribution since only the retarded Green's function is of our concern.

Fix the momentum at $k_F^*$, the (retarded) Green function at finite frequency and finite temperature takes the form

$$\begin{aligned} G_c(k_F,\, \omega,\, T) &= \frac{1}{\omega - i\,\text{Im}\Sigma(k_F, \omega)} = \frac{1}{\omega - i\,\alpha T} \\ &= T^{-1} g\left(k_F^*, \frac{\omega}{T}\right). \end{aligned} \tag{I.33}$$

In Eq. (I.33) $\alpha = \frac{2\pi\, J_\chi^2\, \epsilon_\chi^*}{\bar{\lambda}^3}$ and $g\left(k_F^*, \frac{\omega}{T}\right)$ is the scaling function for $G_c$ in terms of $\omega/T$, obeying the $\omega/T$-scaling behavior.

---


[1] Lijun Zhu, and Q. Si, Phys. Rev. B **66**, 024426 (2002).

[2] Q. Si, S. Rabello, K. Ingersent, and J. Smith, Phys. Rev. B **68**, 115103 (2003).

[3] P. Coleman, Phys. Rev. B **29**, 3035 (1984).

[4] J. Ye, and S. Sachdev, Phys. Rev. B **44**, 18 (1991).

[5] S. J. Yamamoto, and Q. Si, Phys. Rev. B **81**, 1–15 (2010).

[6] S. Paschen, Silke, T. Lühmann, S. Wirth, P. Gegenwart, O. Trovarelli, C. Geibel, F. Steglich, P. Coleman, and Q. Si, Nature **432**, 881-885 (2004).

[7] S. Friedemann, N. Oeschler, S. Wirth, C. Krellner, C.Geibel, F. Steglich, S. Paschen, S. Kirchner, and Q. Si, PNAS **107**, 14547-51 (2010).

[8] A. Rosch, J. Paaske, J. Kroha, and P. Wölfle, J. of the Phys. Soc. of Japan **74**, 118–126 (2005).

[9] A. Rosch, J. Paaske, J. Kroha, and P. Wölfle, Phys. Rev. Lett. **90**, 076804 (2003).

[10] P. Coleman, in *Heavy fermions: Electrons at the edge of magnetism* ( Cambridge University Press, Cambridge, England, 2015).

[11] J. Custers, P. Gegenwart, H. Wilhelm, K. Neumaier, Y. Tokiwa, O. Trovarelli, C. Geibel, F. Steglich, C. Ppin, and P. Coleman, Nature **424**, 524-527 (2003).

[12] J. Custers, P. Gegenwart, C. Geibel, F. Steglich, P. Cole- man, and S. Paschen, Phys. Rev. Lett. **104**, 186402 (2010).

[13] J. Hertz, Phys. Rev. B **14**, 1165-1184 (1976).

[14] A. J. Millis, Phys. Rev. B **48**, 7183 (1993).

[15] H. v. Löhneysen, A. Rosch, M. Vojta, and P. Wölfle, Peter, Rev. Mod. Phys. **79**, 1015 (2007).

[16] M. Vojta, and L. Fritz, Phys. Rev. B **70**, 094502 (2004).

[17] A. C. Hewson, in *The Kondo problem to heavy fermions* (Cambridge university press, Cambridge, England, 1997).

[18] O. Trovarelli, J. Custers, P. Gegenwart, C. Geibel, P. Hinze, S. Mederle, G. Sparn, and F. Steglich, Physica B: Condens. Matter **312**, 401- 402 (2002).

[19] P. Gegenwart, J. Custers, T. Tayama, K. Tenya, C. Geibel, O. Trovarelli, and F. Steglich, Acta. Phys. Pol. B **34**, 323334 (2003).
